# Supplementary material for: TRIAD: a triple patterning lithography aware detailed router
Source: arXiv:1402.2906 source file (2014-02-12)
Supplement: Supplementary file 1 [file supplement.tex]

\section{Supplemental Material}

\subsection{Details of Detailed Routing}
 Lee algorithm \footnote{\small{C. Y. Lee, "An Algorithm for Path Connection and its Application," \textit{IRE Trans. on Electronic Computers}, EC-10, 1961.}} is the most well known routing method to find a connection from a source point to a target point.
 Lee algorithm-based routers contain two main stages for each route: \textit{propagation} and \textit{retracing}.
 In the propagation stage, the router iteratively explores adjacent routing units to approach the target point.
 Each propagation step also records the routing cost.
 After reaching the target point, the routing connection is generated by retracing the propagation order on the grid map.

\subsection{Innovative Conflict Graph}
Lin and Li \cite{DPL_Lin_DAC10} proposed an \textit{innovative conflict graph} (ICG) based on \cite{DPL_Kahng_TCAD10} to enable detailed routers to escape the suboptimum of coloring caused by a greedy assignment.
ICG contains \textit{determined} and \textit{undetermined vertices} to represent routed and routing wire segments, respectively.
An edge in ICG indicates the spacing of the wire segments represented by its terminal vertices is smaller than $sp_dp$.
Notably, there are \textit{determined} and \textit{undetermined edges} in ICG to represent the DPL relation between routed/routing and routed/routed wire segments.
Each determined vertex is assigned a pseudo color to represent the potential color.
An ICG comprises several innovative conflict subgraphs (ICSGs), and two ICSGs have no determined and undetermined edges between them.
An odd-length cycle in ICG indicates a coloring conflict.
Figure \ref{fig:icg} shows a routing result and its ICG where solid/dashed border rectangles represent routed/routing wires, solid/dashed border circles represent determined/undetermined vertices, and solid/dashed lines represent determined/undetermined edges.
Each determined vertex is assigned a pseudo color to represent the potentially final color.
This work adopts the concept of ICG to implement the insertion of vertices and edges in TECG caused by routing wire segments.

\begin{figure}[h]
	\centering
	\subfloat[]{\includegraphics[width=0.18\textwidth]{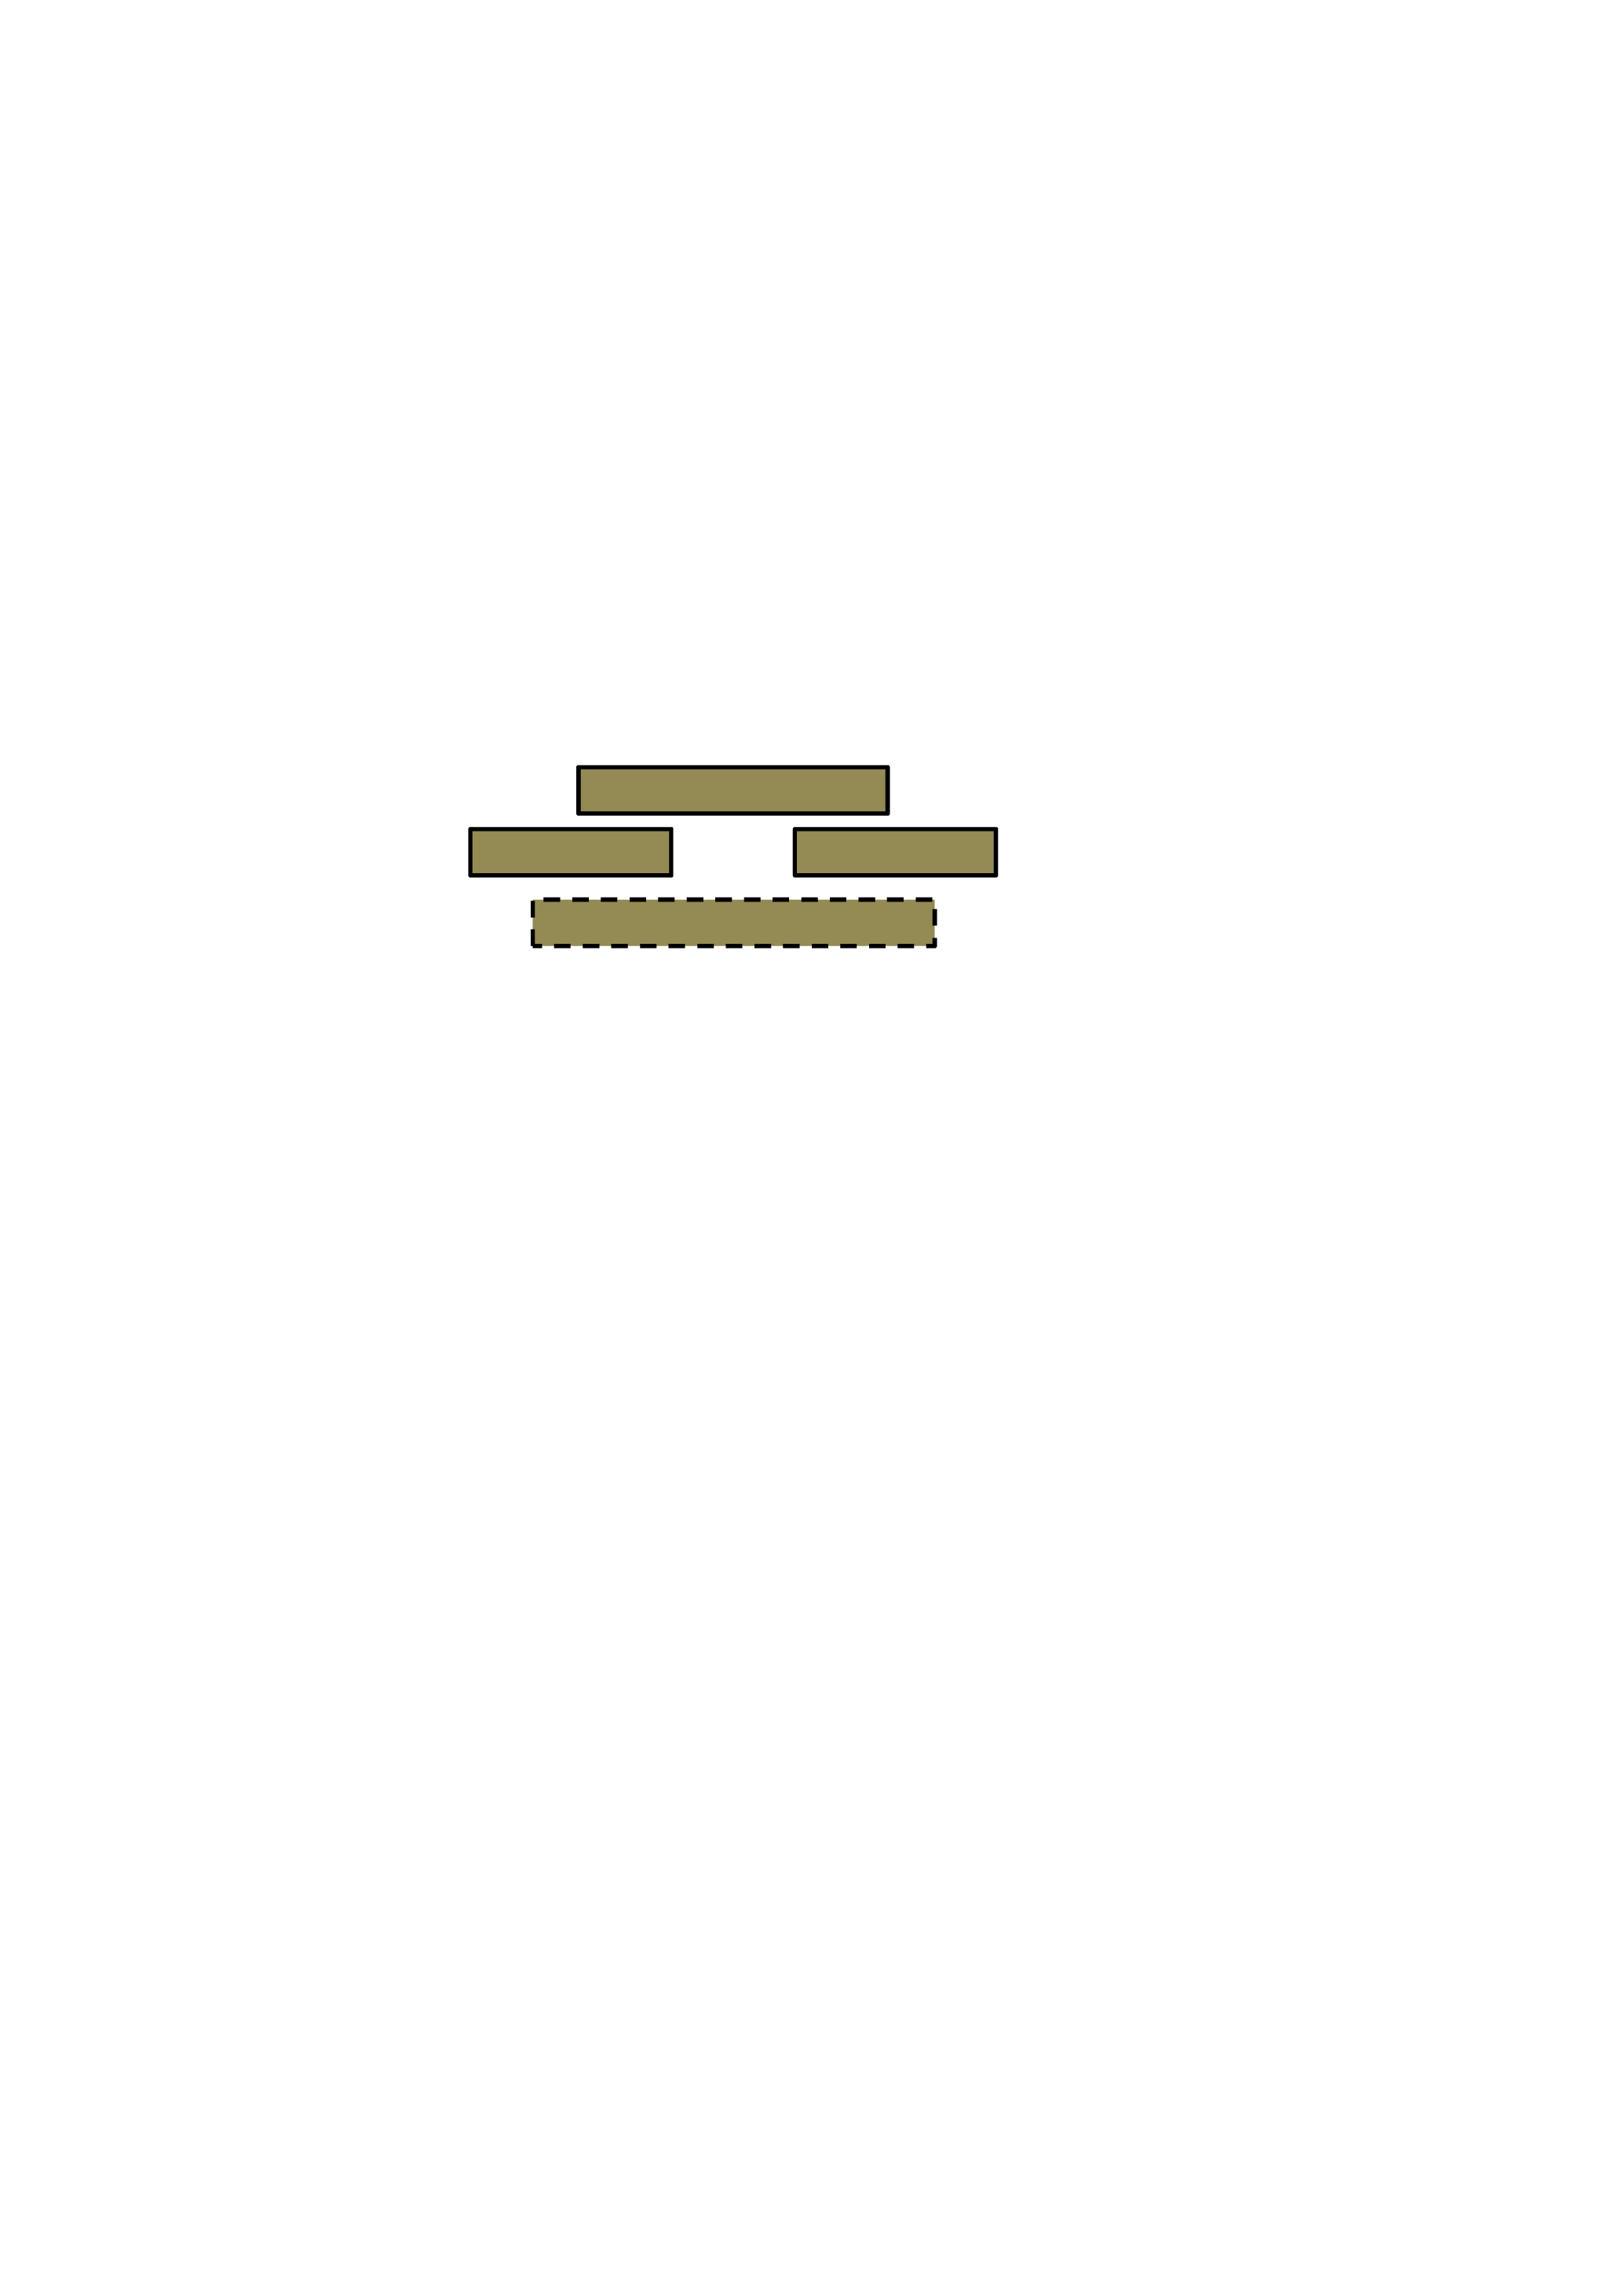}}
    \hspace{0.04\textwidth}
	\subfloat[]{\includegraphics[width=0.18\textwidth]{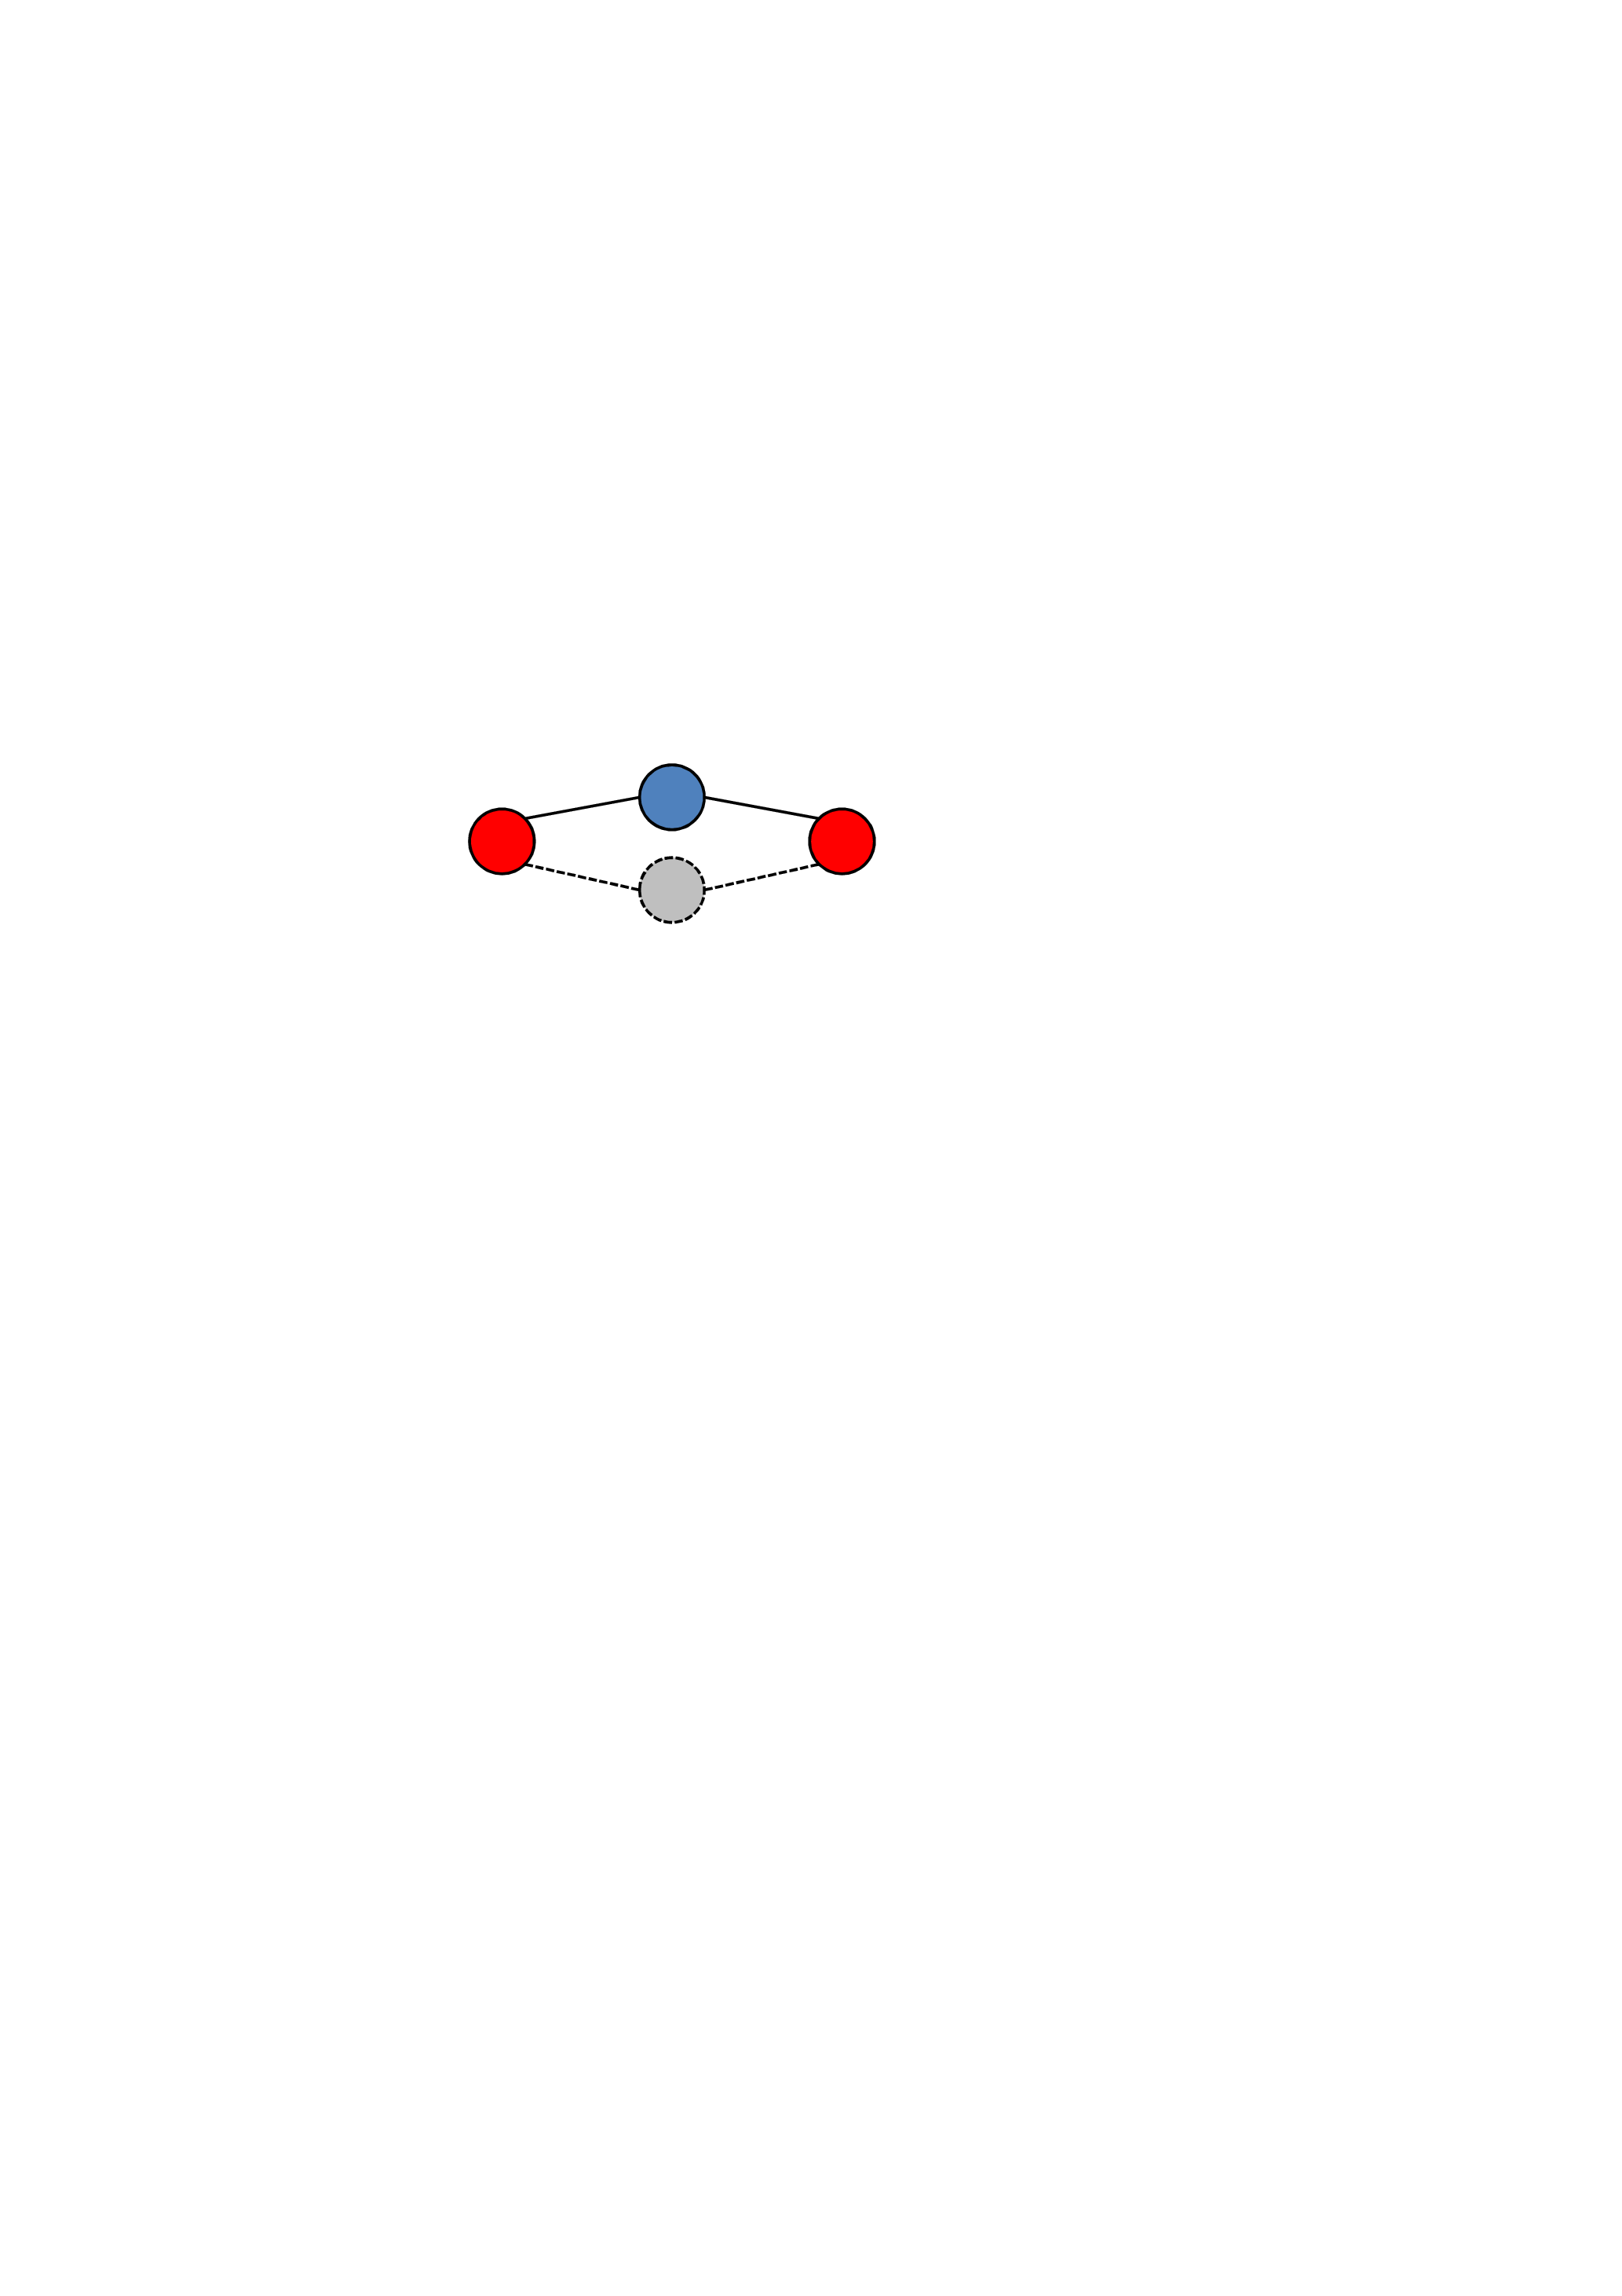}}
	\caption{Example of ICG: (a) layout contains three routed wires and one wire to be routed; (b) ICG of (a).}
	\label{fig:icg}
\end{figure}
