# Supplementary material for: TRIAD: a triple patterning lithography aware detailed router
Source: arXiv:1402.2906 source file (2014-02-12)
Supplement: Supplementary file 2 [file supplement1.tex]

\subsection{Rip-up Operation of TECG}

Rip-up and re-route is a necessary means to accomplish detailed routing when some nets cannot be routed successfully.
Due to the page limitation, we skip the rip-up operation of TECG in the main article.
Detailed routers rip up routed wire segments to release routing resource for unroutable nets.
After ripping up one wire segment, the corresponding vertex $v^c$ in CG needs to be removed from CG, which requires disconnecting $v^c$ and $v^c_i \in V^\mathcal{C}_{ad}(v^c)$.
Without loss of generality, two disconnected tokens $T_w \in V^\mathcal{T}$ and $T_x \in V^\mathcal{T}$ are merged into $T_{mrg}$ when the following two conditions are satisfied.
\begin{enumerate}
  \item There exists one SCC $scc = (T_x, T_y, T_z)$ in $\mathcal{G^T}$, and
  \item $T_w$ connects to $T_y$ and $T_z$.
\end{enumerate}
Then $scc$ is updated as $scc_{mrg} = (T_{mrg}, T_y, T_z)$.
Disconnecting two vertices in CG may break one of the two merging conditions, resulting in \textit{token splitting}.
Figure \ref{fig:s_tecg_ripup}(a) depicts one TECG containing one SCC $scc=(T_2, T_3, T_4)$.
Connecting $A$ and $B$ makes $T_1$ and $T_4$ be merged into $T_5$ as shown in Fig. \ref{fig:s_tecg_ripup}(b).
After disconnecting $B$ and $C$, $token(B) = T_2$ and $token(C) = T_3$ is also disconnected in TG, resulting in the destruction of $scc$.
Notably, $token(A)$ and $token(D)$ are identical due to the appearance of $scc$.
When $scc$ is destructed, $token(A)$ and $token(D)$ differ by splitting $T_5$ into $T_6$ and $T_7$ as shown in Fig. \ref{fig:s_tecg_ripup}(c).
To facilitate token splitting, \textit{merging edges} in CG are generated when two tokens are merged.
The merging edge generation and removal are introduced followed by token splitting.

\begin{figure}[tb!]
	\centering
	\subfloat[]{\includegraphics[width=0.15\textwidth]{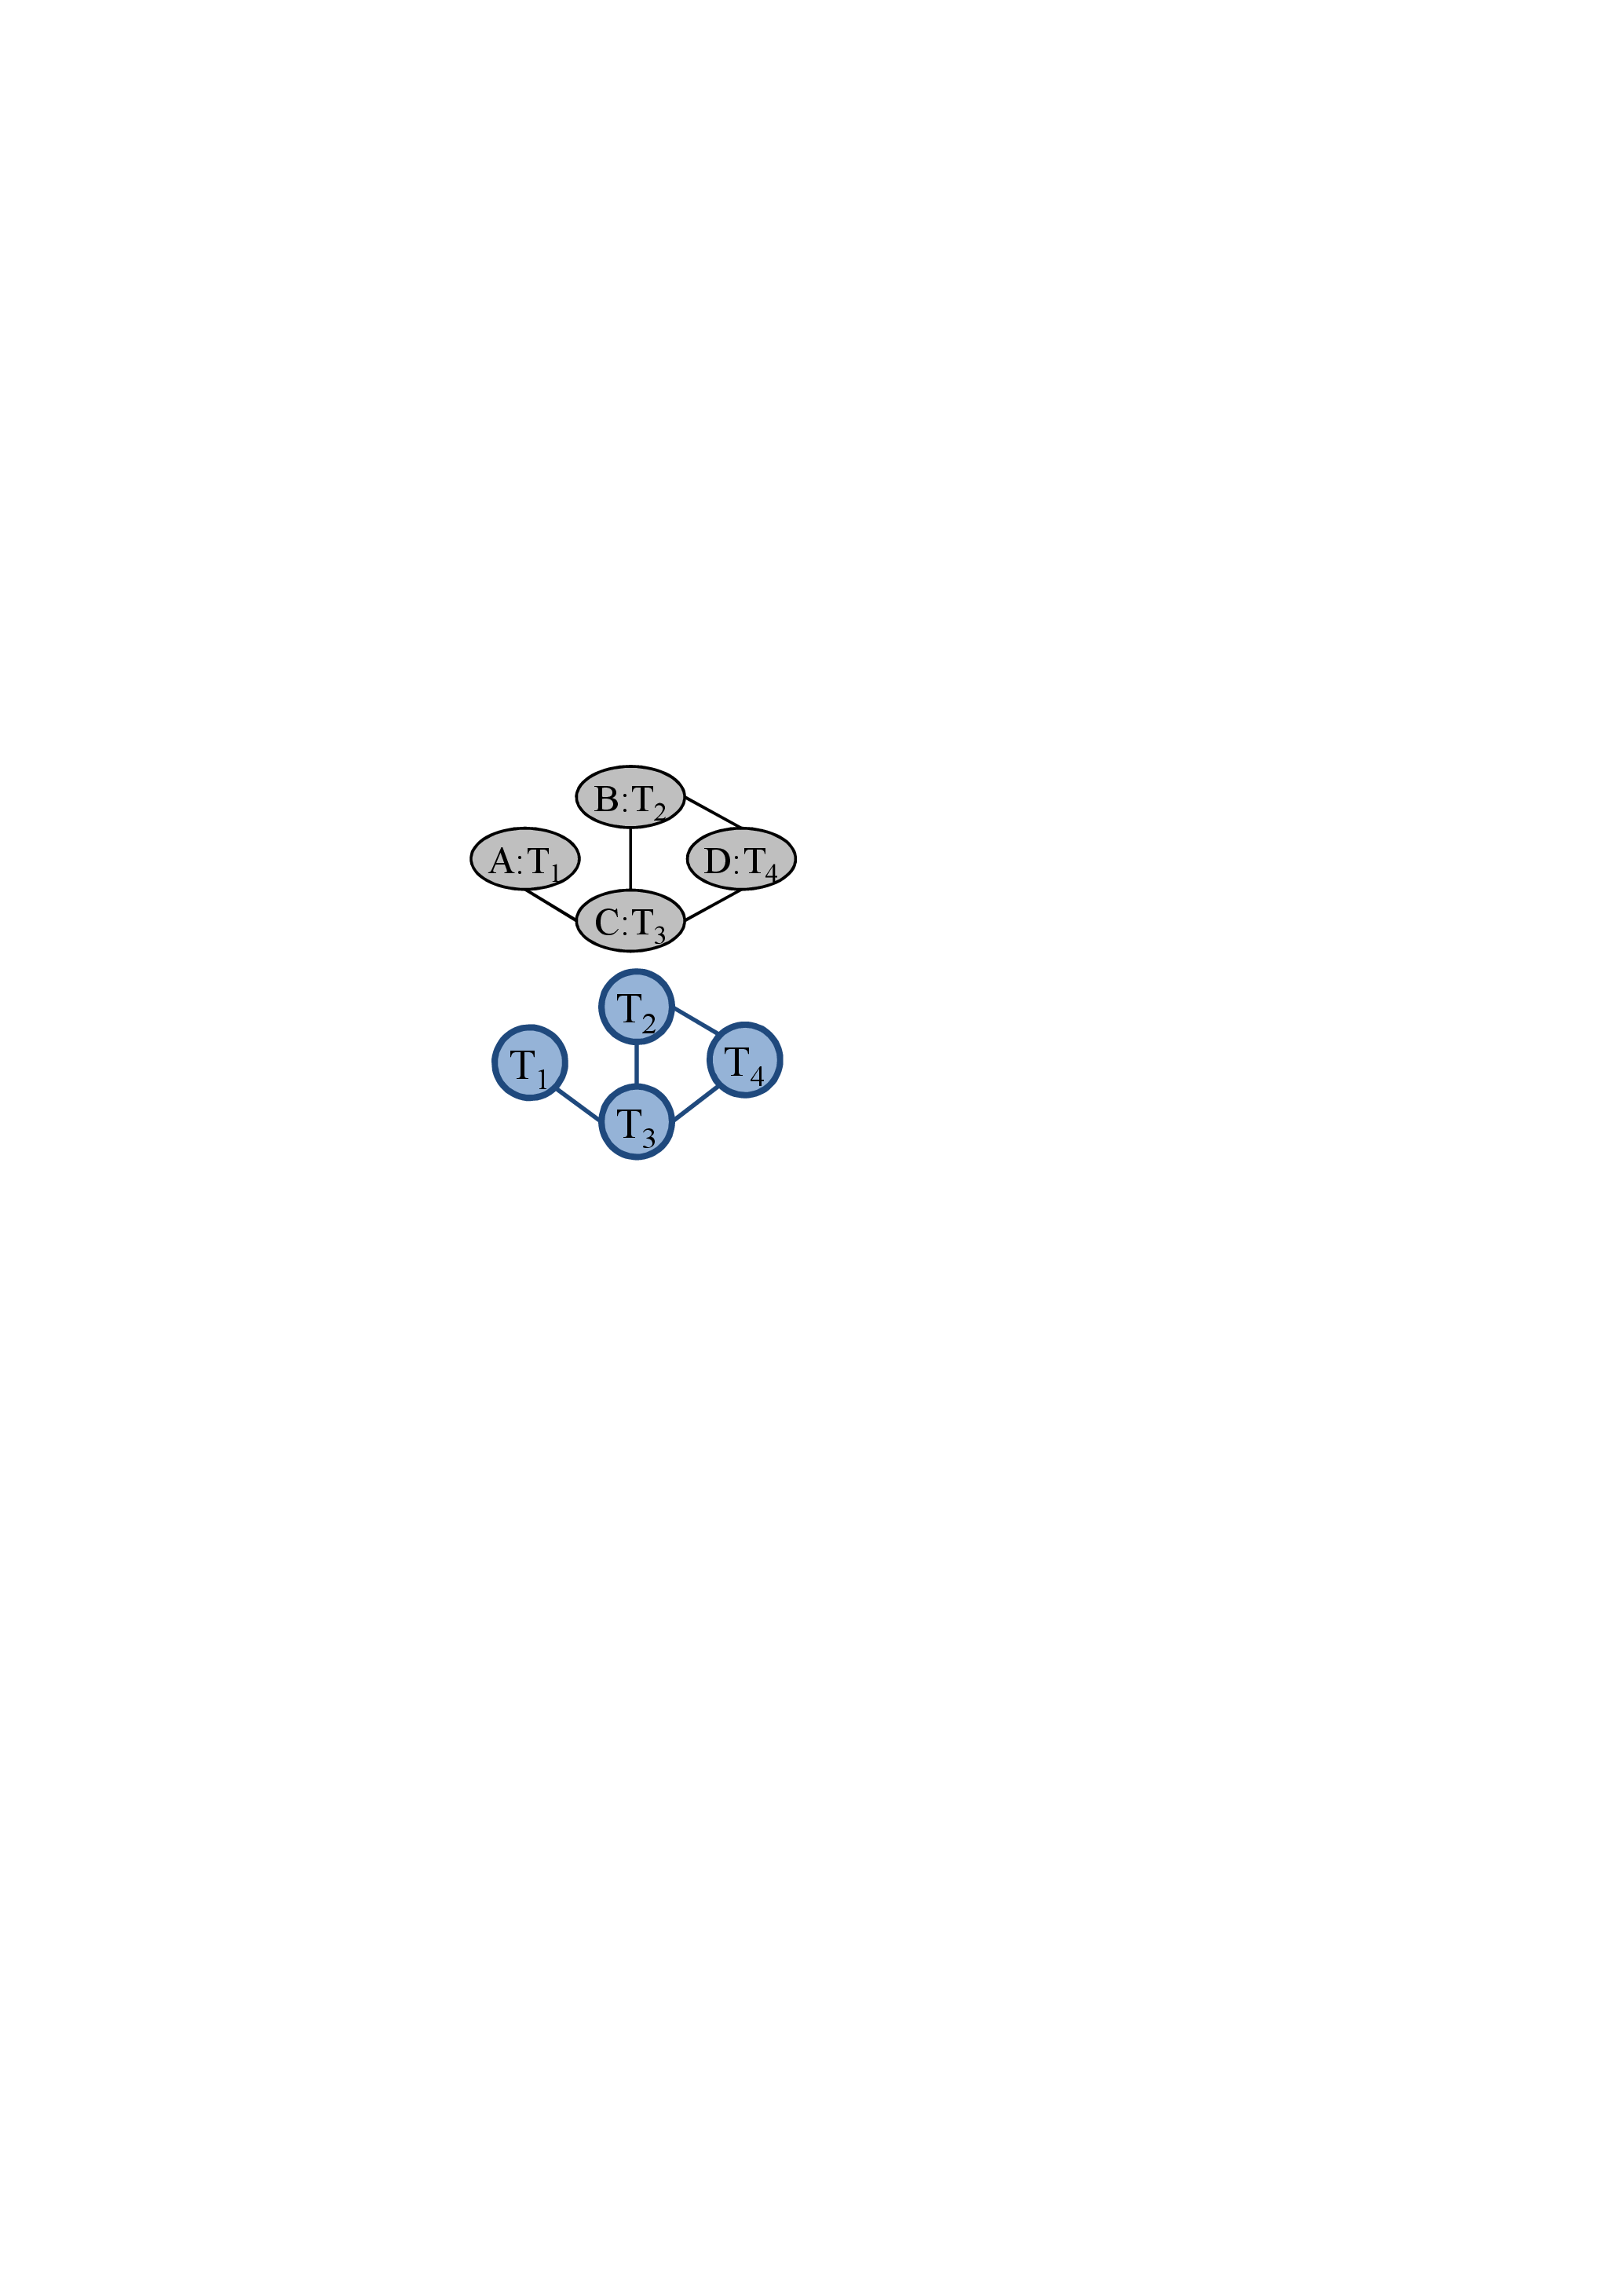}}
	%\subfloat[]{\includegraphics[height=0.08\textheight]{fig/s_tecg_bf_ripup0.eps}}
    %\hspace{0.001\textwidth}
	\subfloat[]{\includegraphics[width=0.15\textwidth]{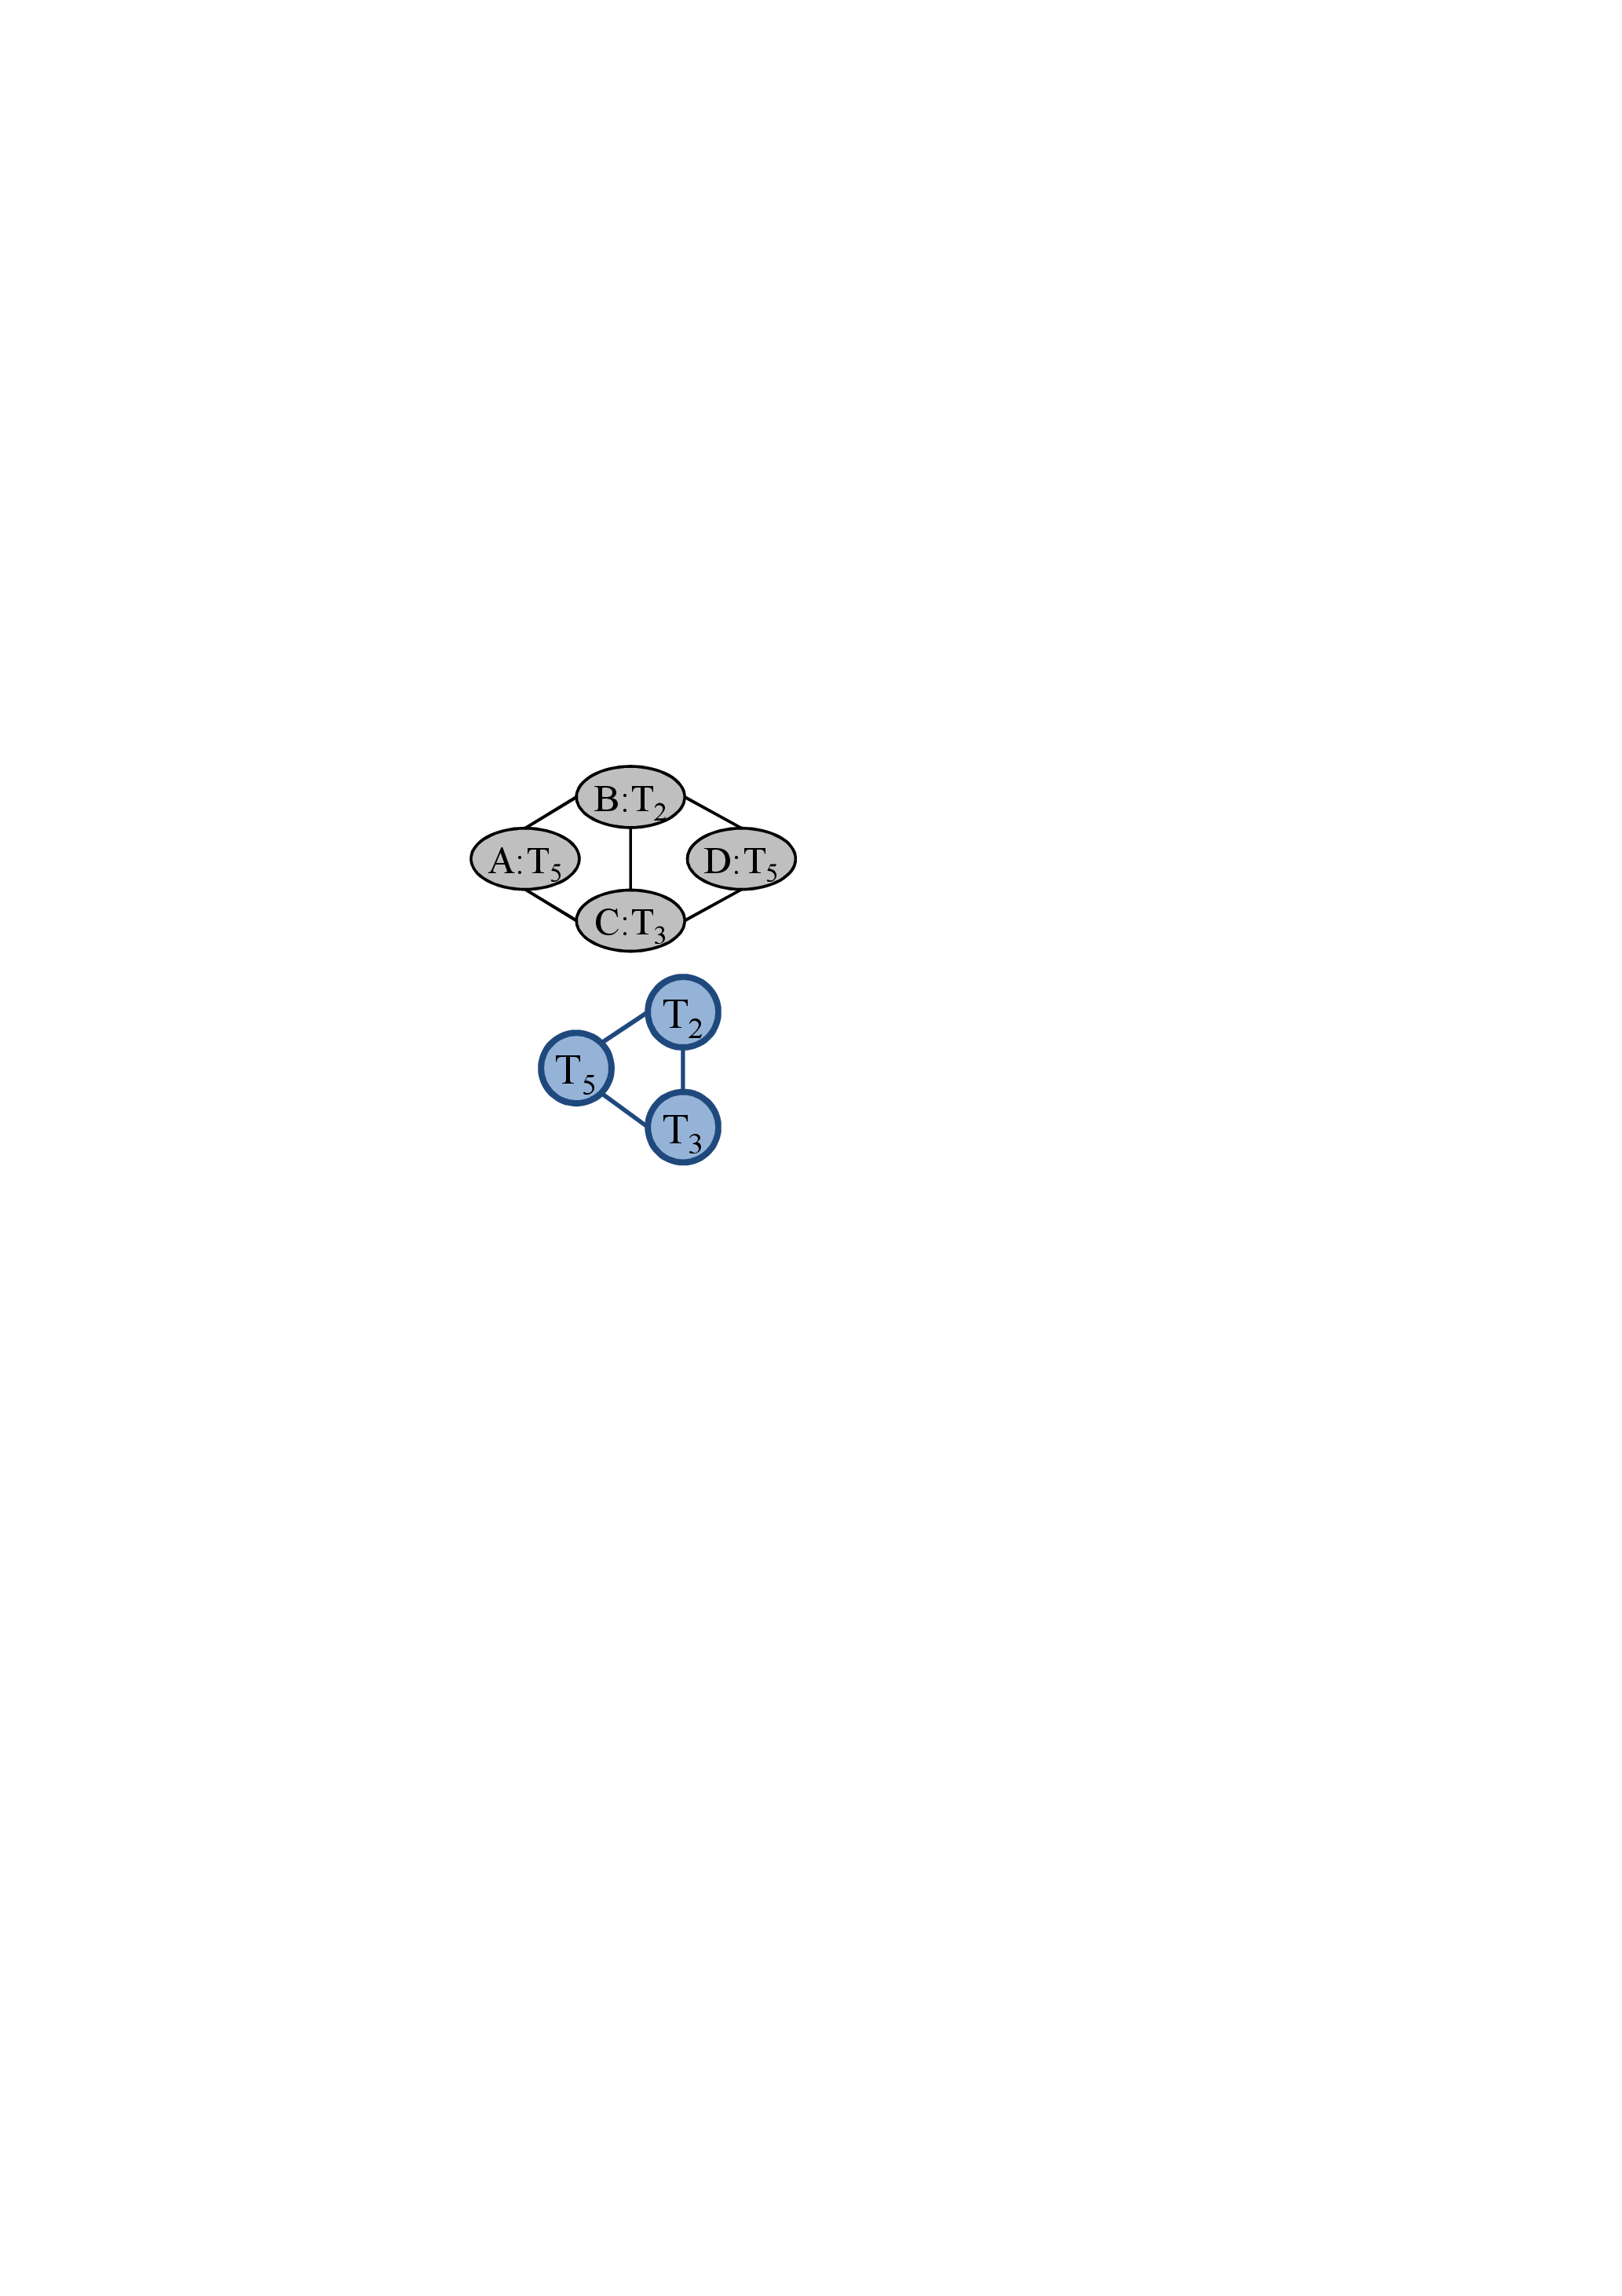}}
	%\subfloat[]{\includegraphics[height=0.08\textheight]{fig/s_tecg_bf_ripup.eps}}
    %\hspace{0.001\textwidth}
	\subfloat[]{\includegraphics[width=0.15\textwidth]{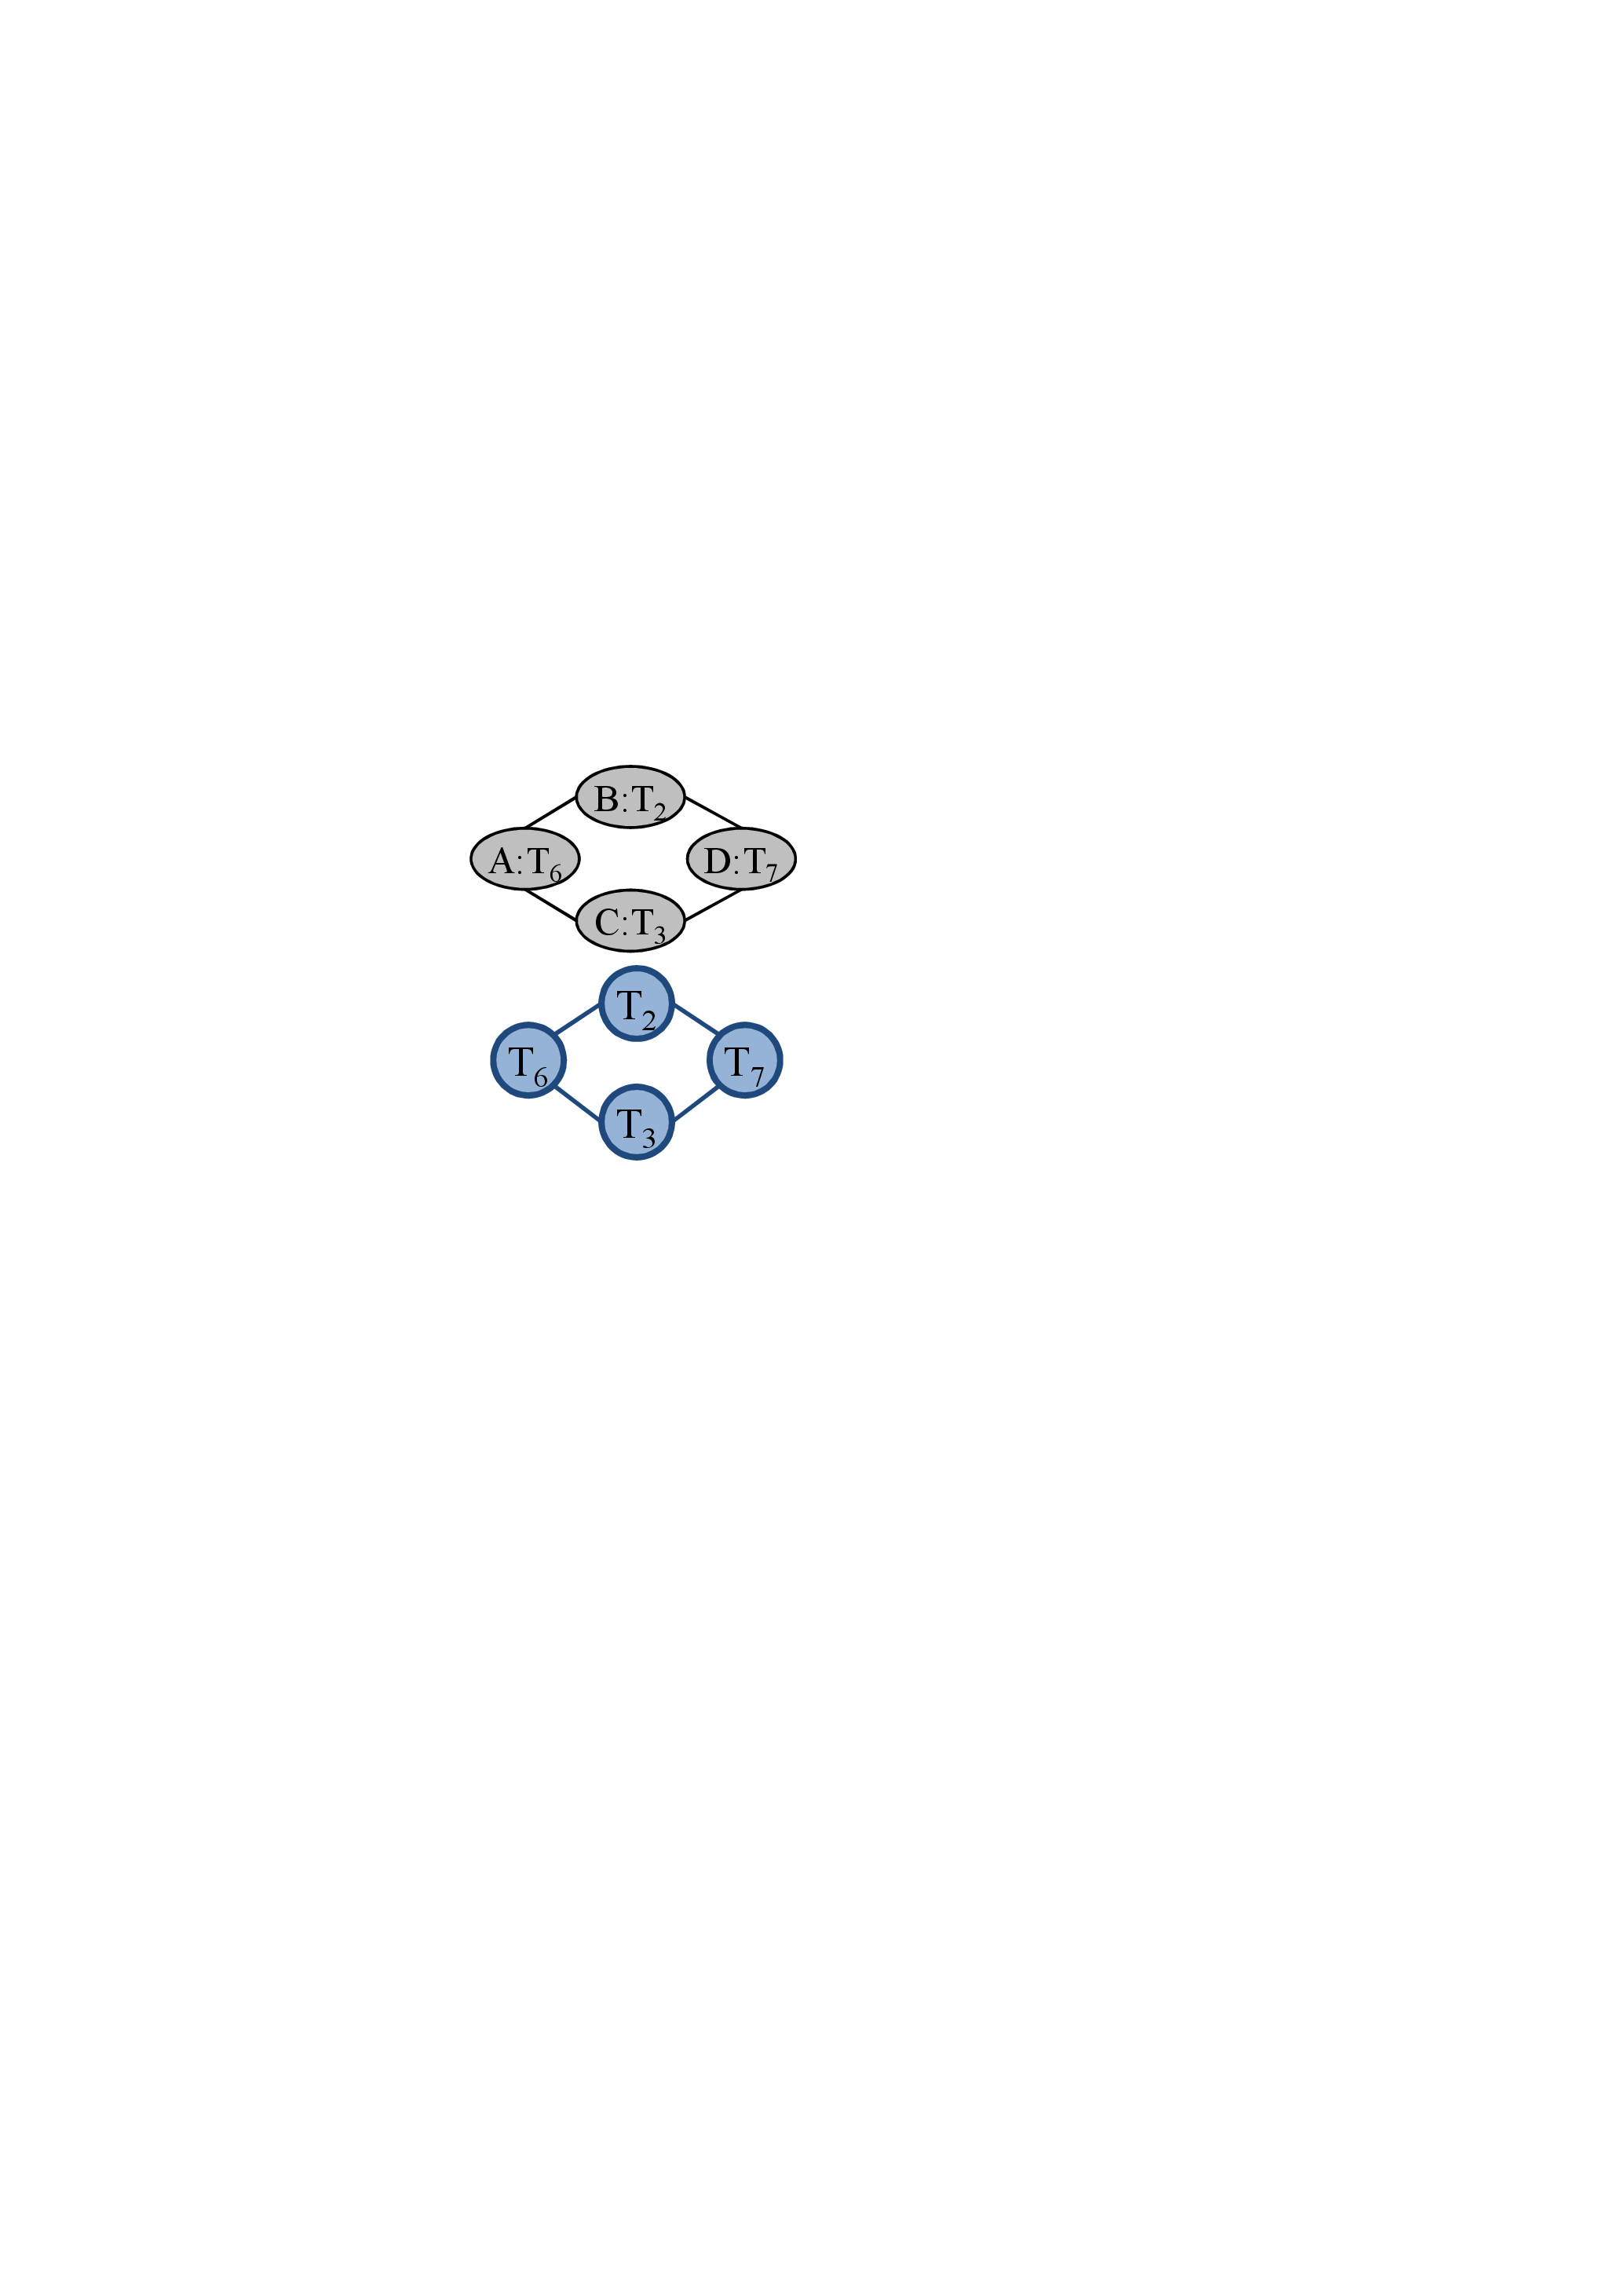}}
	%\subfloat[]{\includegraphics[height=0.08\textheight]{fig/s_tecg_af_ripup.eps}}
	\caption{TECG after rip-up: (a) TECG before connecting $A$ and $B$ in CG; (b) updated TECG; (c) TECG after disconnecting $B$ and $C$ in CG.}
	\label{fig:s_tecg_ripup}
\end{figure}

\subsubsection{Merging Edge Generation}
Merging two tokens $T_w \in V^\mathcal{T}$ and $T_x \in V^\mathcal{T}$ into $T_{mrg}$ reassigns $token(v^c)$ as $T_{mrg}$ where $v^c \in V^\mathcal{C}_t(T_w) \cup V^\mathcal{C}_t(T_x)$.
Before merging $T_w$ and $T_x$, \textit{merging edges} are generated between $V^\mathcal{C}_t(T_w)$ and $V^\mathcal{C}_t(T_x)$.
Before introducing merging edge generation, \textit{merging pattern} is firstly defined as follows.

\begin{define}[\textbf{Merging Pattern}]
%Assume that $T_w$ and $T_x$ are being merged into $T_{mrg}$ with one SCC $scc = (T_x, T_y, T_z)$.
A merging pattern in CG is defined as a four-tuple $(v^c_{cnt1}$, $v^c_{cnt2}$, $v^c_{brdg1}$, $v^c_{brdg2})$ where $token(v^c_{cnt1})$ = $T_w$ and $token(v^c_{cnt2})$ = $T_x$ are being merged, $token(v^c_{brdge1}) = T_y$, $token(v^c_{brdge2})$ = $T_z$, and there exists one SCC $scc = (token(v^c_{cnt2})$, $token(v^c_{brdg1})$, $token(v^c_{brdg2}))$ in TG.
\end{define}

%A merging pattern indicates that $token(v^c_{cnt1})$ and $token(v^c_{cnt2})$ are merged because $v^c_{cnt1}$ and $v^c_{cnt2}$ connect to $v^c_{brdg1}$ and $v^c_{brdg2}$.

Algorithm \ref{alg:s_MP_generation} shows the algorithm of merging pattern generation before two tokens $T_w$ and $T_x$ are merged.
Firstly, a merging pattern set $S^{MP}$ is set as empty.
Each vertex $v^c_w \in V^\mathcal{C}_t(T_w)$ tries to generate merging patterns with vertex $v^c_x \in V^\mathcal{C}_t(T_x)$.
Two adjacent vertices of $v^c_w$, such as $v^c_{ad1} \in V^\mathcal{C}_{ad}(v^c_w)$ and $v^c_{ad2} \in V^\mathcal{C}_{ad}(v^c_w)$ where $token(v^c_{ad1}) = T_y$ and $token(v^c_{ad2}) = T_z$, are identified.
Then the adjacent vertex of $v^c_{ad1}$, such as $v^c_{adx} \in V^\mathcal{C}_{ad}(v^c_{ad1})$ where $token(v^c_{adx}) = T_x$, is found to generate one merging pattern with $v^c_w$, $v^c_{ad1}$, and $v^c_{ad2}$ (lines 2--9).
%Similarly, Each vertex $v^c_x \in V^\mathcal{C}_t(T_x)$ tries to generate one merging pattern with vertex $v^c_w \in V^\mathcal{C}_t(T_w)$ (lines 10--17).

\begin{algorithm}[bt!]
\caption{Merging Pattern Generation}
\label{alg:s_MP_generation}
\begin{algorithmic}[1]
  \REQUIRE Two tokens $T_w \in V^\mathcal{T}$ and $T_x \in V^\mathcal{T}$ to be merged, one SCC $scc$ = $(T_x, T_y, T_z)$
  \STATE Merging pattern set $S^{MP} := \emptyset$;
  \FORALL {$v^c_w \in V^\mathcal{C}_t(T_w)$}
    \FORALL {$v^c_{ad1} \in V^\mathcal{C}_{ad}(v^c_w)$, $v^c_{ad2} \in V^\mathcal{C}_{ad}(v^c_w)$ where $token(v^c_{ad1})$ = $T_y$, $token(v^c_{ad2})$ = $T_z$}
      \FORALL {$v^c_{adx} \in V^\mathcal{C}_{ad}(v^c_{ad1})$ where $token(v^c_{adx})$ = $T_x$}
        \STATE Generate one merging pattern $mp$ = $(v^c_w$, $v^c_{adx}$, $v^c_{ad1}$, $v^c_{ad2})$;
        \STATE $S^{MP} := S^{MP} \cup \{ mp \}$;
      \ENDFOR
    \ENDFOR
  \ENDFOR
  \RETURN $S^{MP}$;
\end{algorithmic}
\end{algorithm}

One merging pattern $mp$ = $(v^c_{cnt1}$, $v^c_{cnt2}$, $v^c_{brdg1}$, $v^c_{brdg2})$ generates one merging edge, denoted as $e^c_{mrg}(T_mrg)$ between $v^c_{cnt1}$ and $v^c_{cnt2}$ where $T_{mrg}$ is the merging token.
Notably, $v^c_{brdg1}$ and $v^c_{brdg2}$ are called the bridge vertices of $e^c_{mrg}(T_{mrg})$.
Each vertex $v^c \in \mathcal{G^C}$ contains a merging edge set, denoted as $E_{BRDG}(v^c)$, to represent the set of merging edges where $v^c$ is one bridge vertex of $e^c_{mrg} \in E_{BRDG}(v^c)$.
Figure \ref{fig:s_ME}(a) depicts the TECG with merging edges of that in Fig. \ref{fig:s_tecg_ripup}(b) before merging $T_1$ and $T_4$.
After one merging pattern $mp = (A, D, B, C)$ is generated, one merging edge $e_{mrg}$ is generated between $A$ and $D$.
Notably, $B$ and $C$ are the bridge vertices of $e_{mrg}$, resulting in $E_{BRDG}(B) = E_{BRDG}(B) \cup \{e_{mrg}\}$ and $E_{BRDG}(C) = E_{BRDG}(C) \cup \{ e_{mrg}\}$.
Then $T_1$ and $T_4$ are merged into $T_5$ as shown in Fig. \ref{fig:s_ME}(b).

\begin{figure}[bt!]
	\centering
	%\subfloat[]{\includegraphics[height=0.14\textheight]{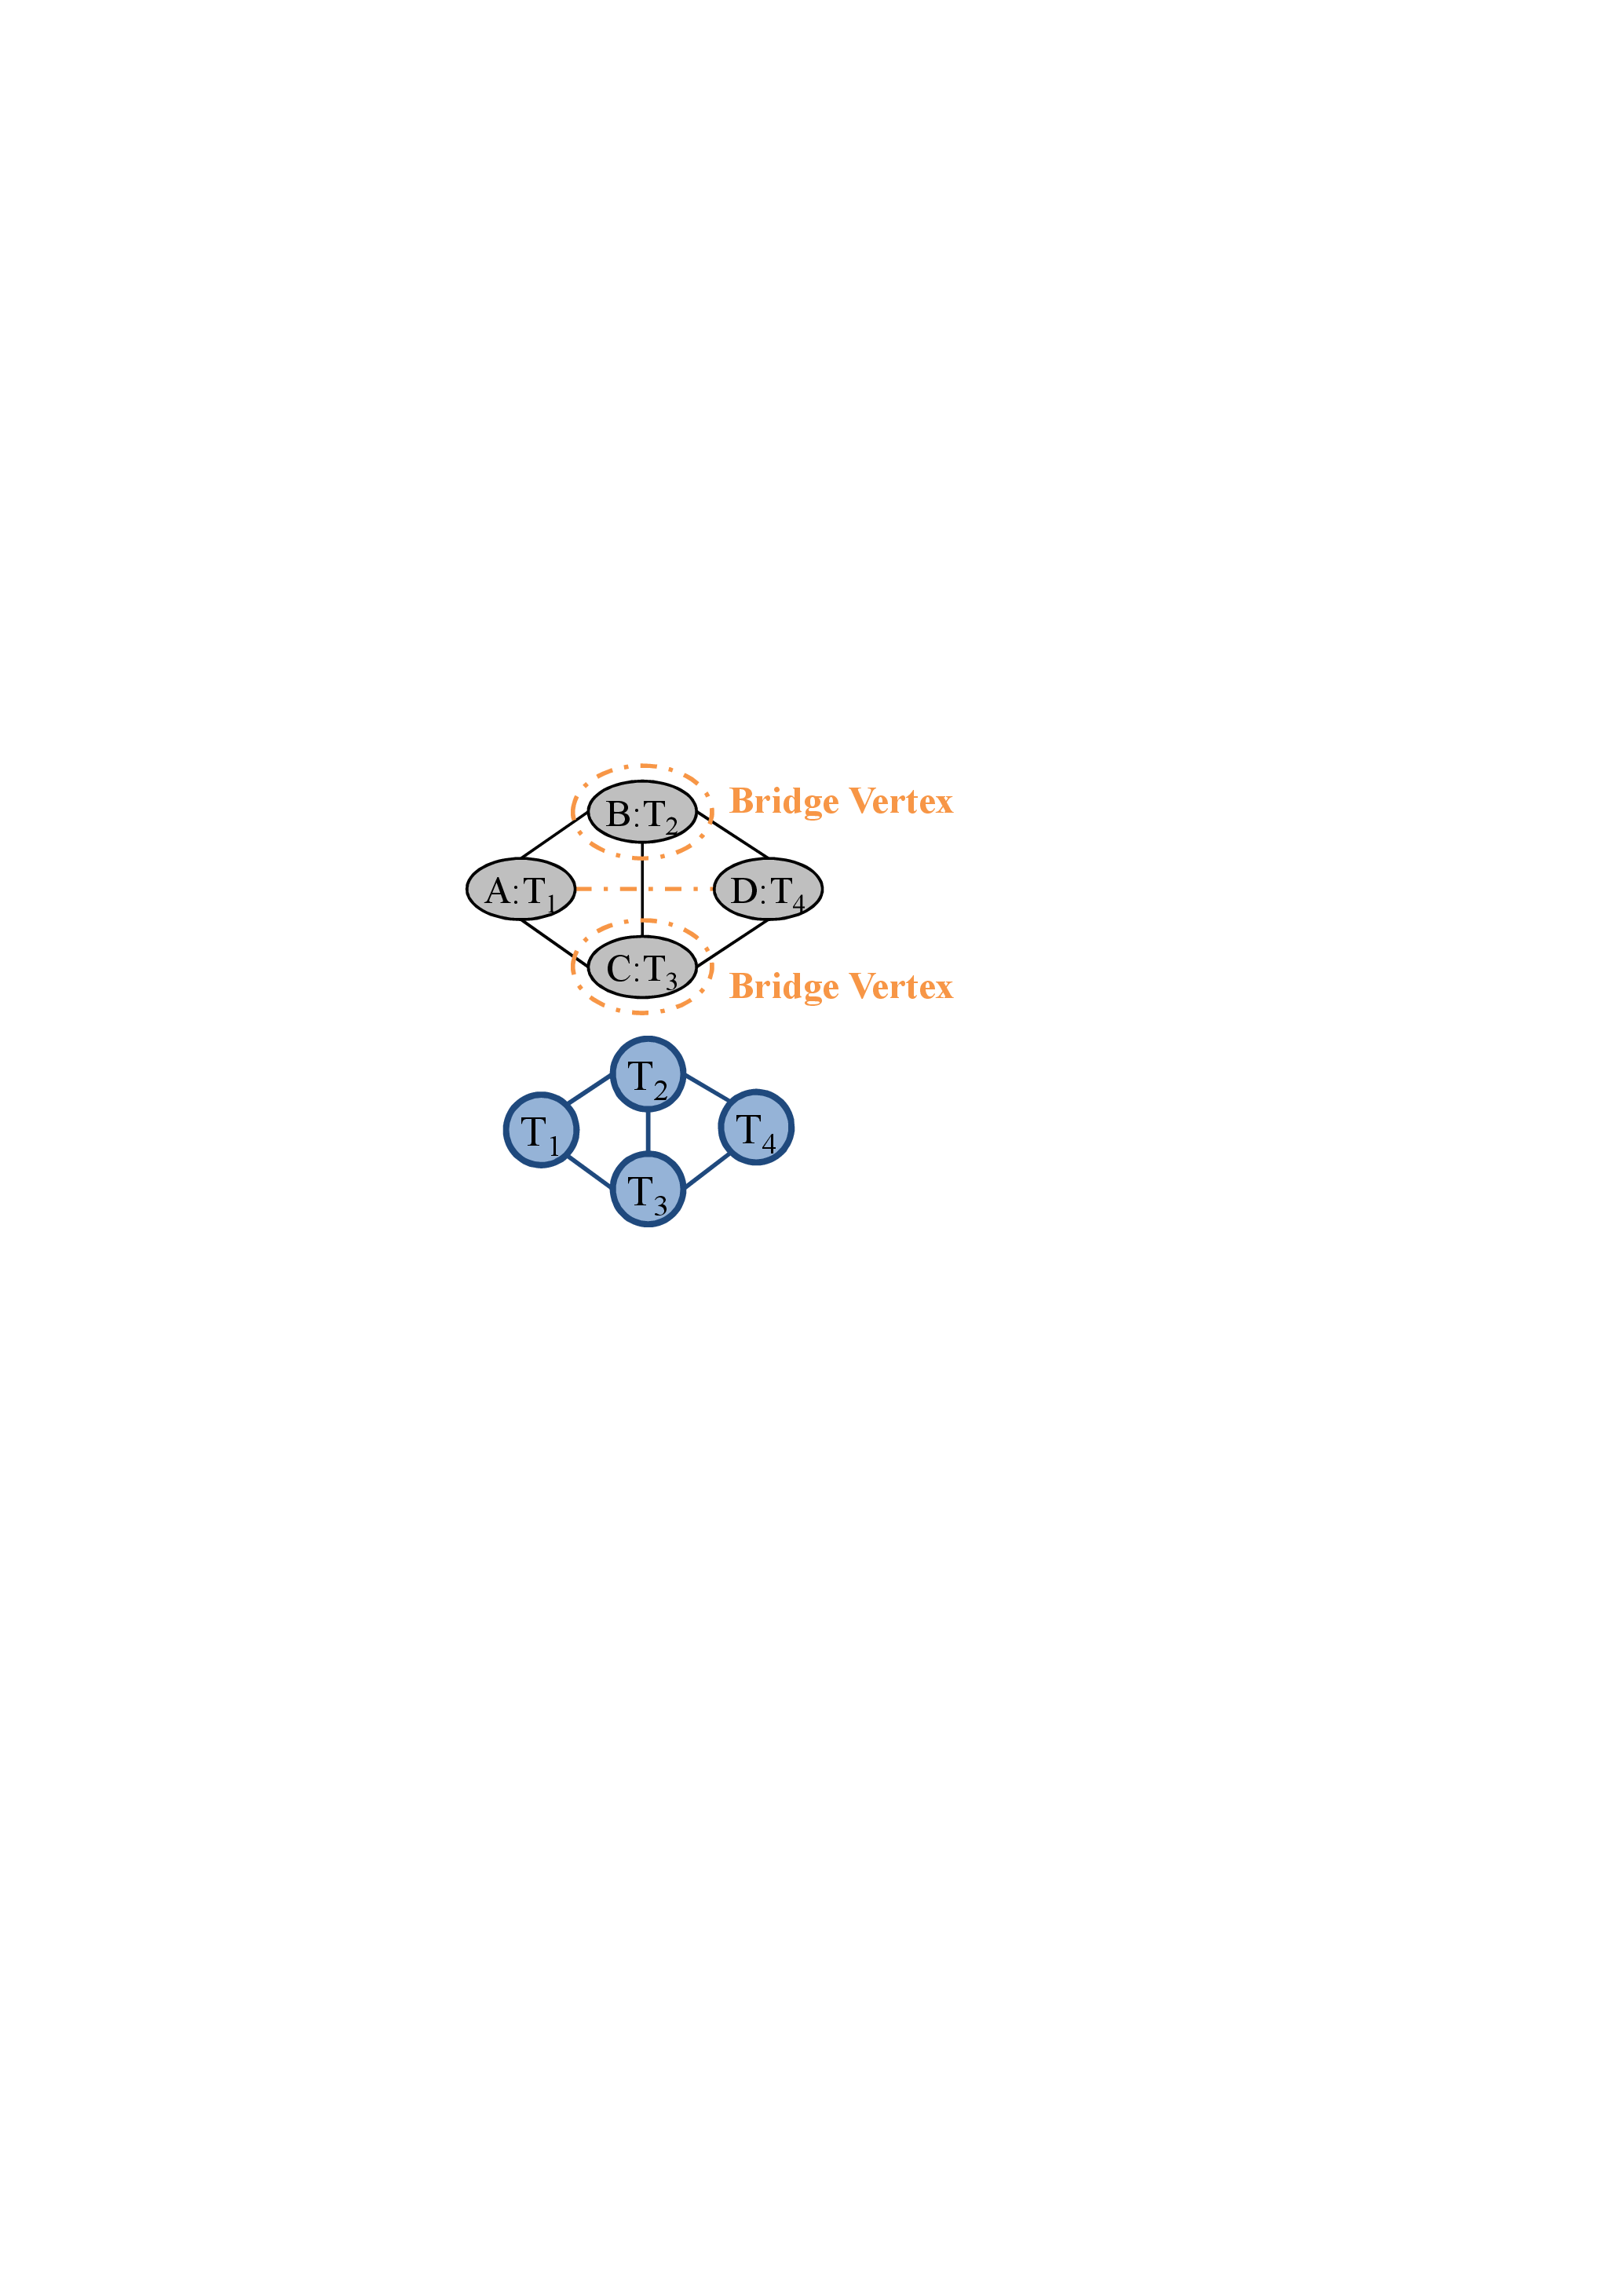}}
    \subfloat[]{\includegraphics[width=0.23\textwidth]{fig/s_ME_bf.eps}}
    %\hspace{0.01\textwidth}
	%\subfloat[]{\includegraphics[height=0.14\textheight]{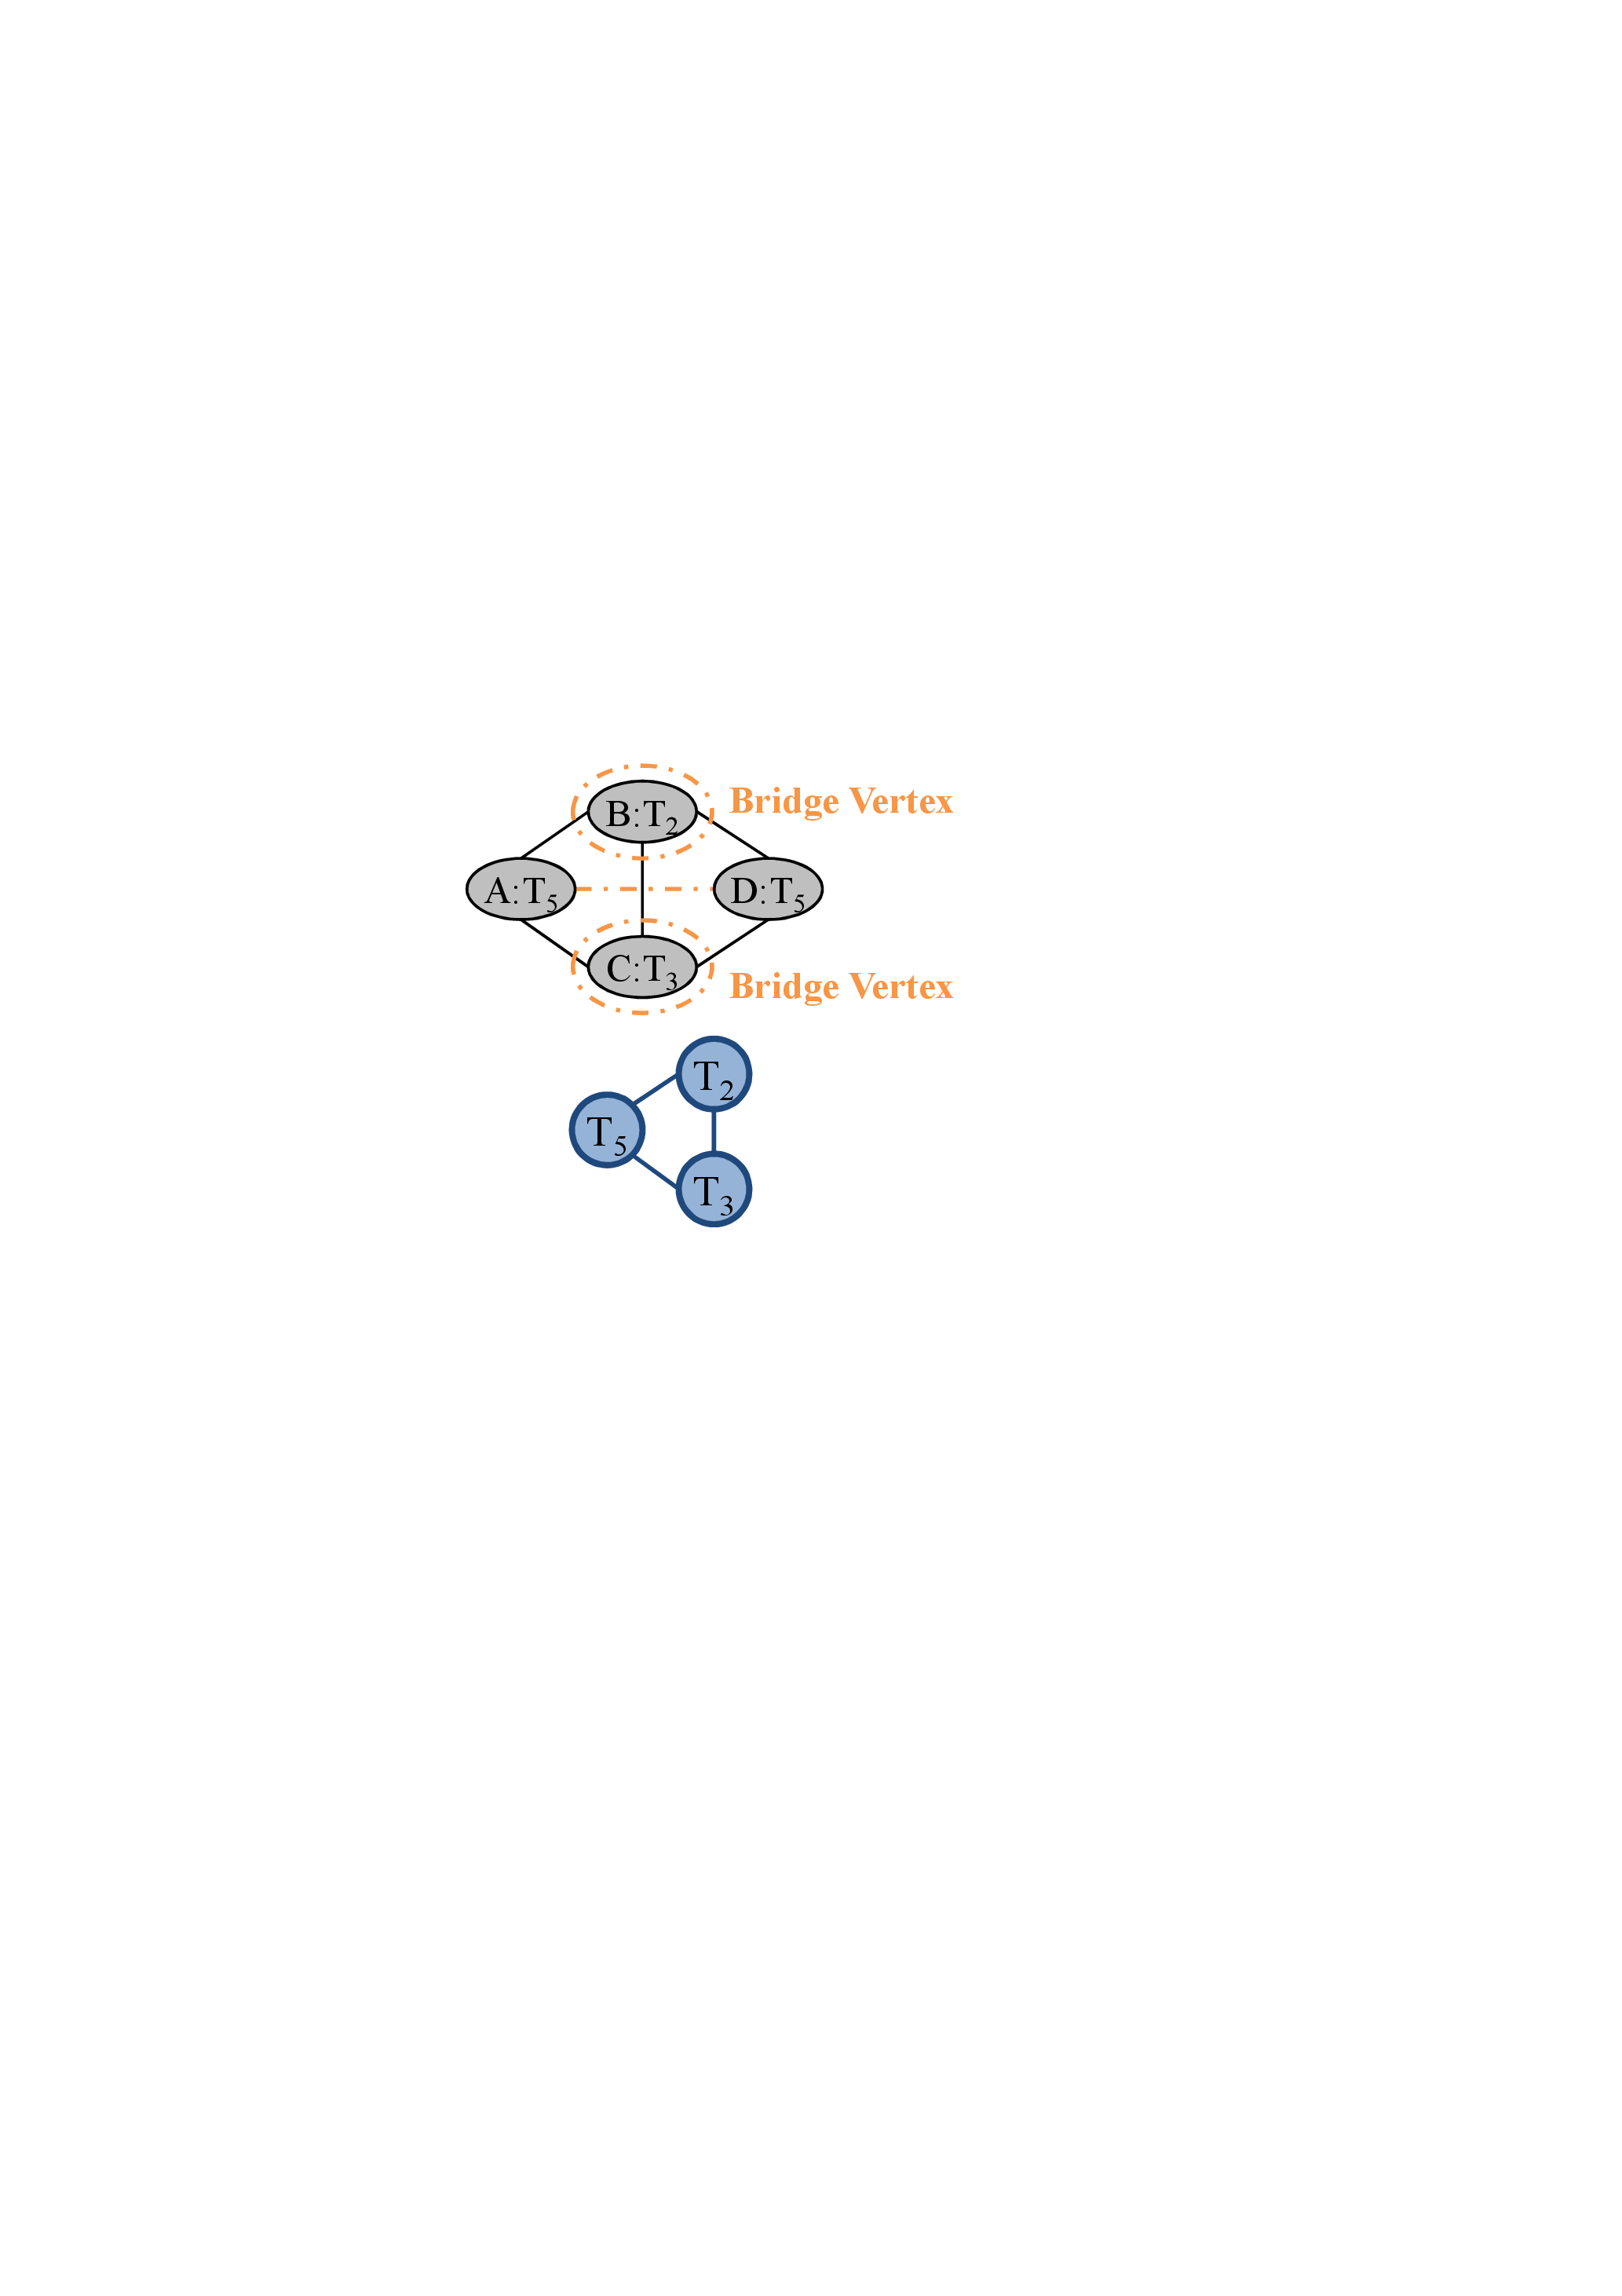}}
	\subfloat[]{\includegraphics[width=0.23\textwidth]{fig/s_ME_af.eps}}
	\caption{Merging pattern and merging edge generation: (a) TECG before merging $tokne(A)$ and $token(D)$; (b) TECG after merging $tokne(A)$ and $token(D)$ into $T_5$.}
	\label{fig:s_ME}
\end{figure}

\subsubsection{Merging Edge Removal}

Removing one vertex $v^c \in V^\mathcal{C}$ requires disconnecting $v^c$ and $v^c_{ad} \in V^\mathcal{C}_{ad}(v^c)$.
One merging pattern  $mp$ = $(v^c_{cnt1}$, $v^c_{cnt2}$, $v^c_{brdg1}$, $v^c_{brdg2})$ is removed when the connection between any vertex pair in $mp$ is removed, if any.
After one merging pattern is removed, the corresponding merging edge is also removed from CG.
Figure \ref{fig:s_MEV}(a)/(b) depicts that the merging edge between $A$ and $D$ in Fig. \ref{fig:s_ME}(b) is removed after disconnecting $A$/$B$ and $C$.

\begin{figure}[bt!]
	\centering
    \subfloat[]{\includegraphics[width=0.16\textwidth]{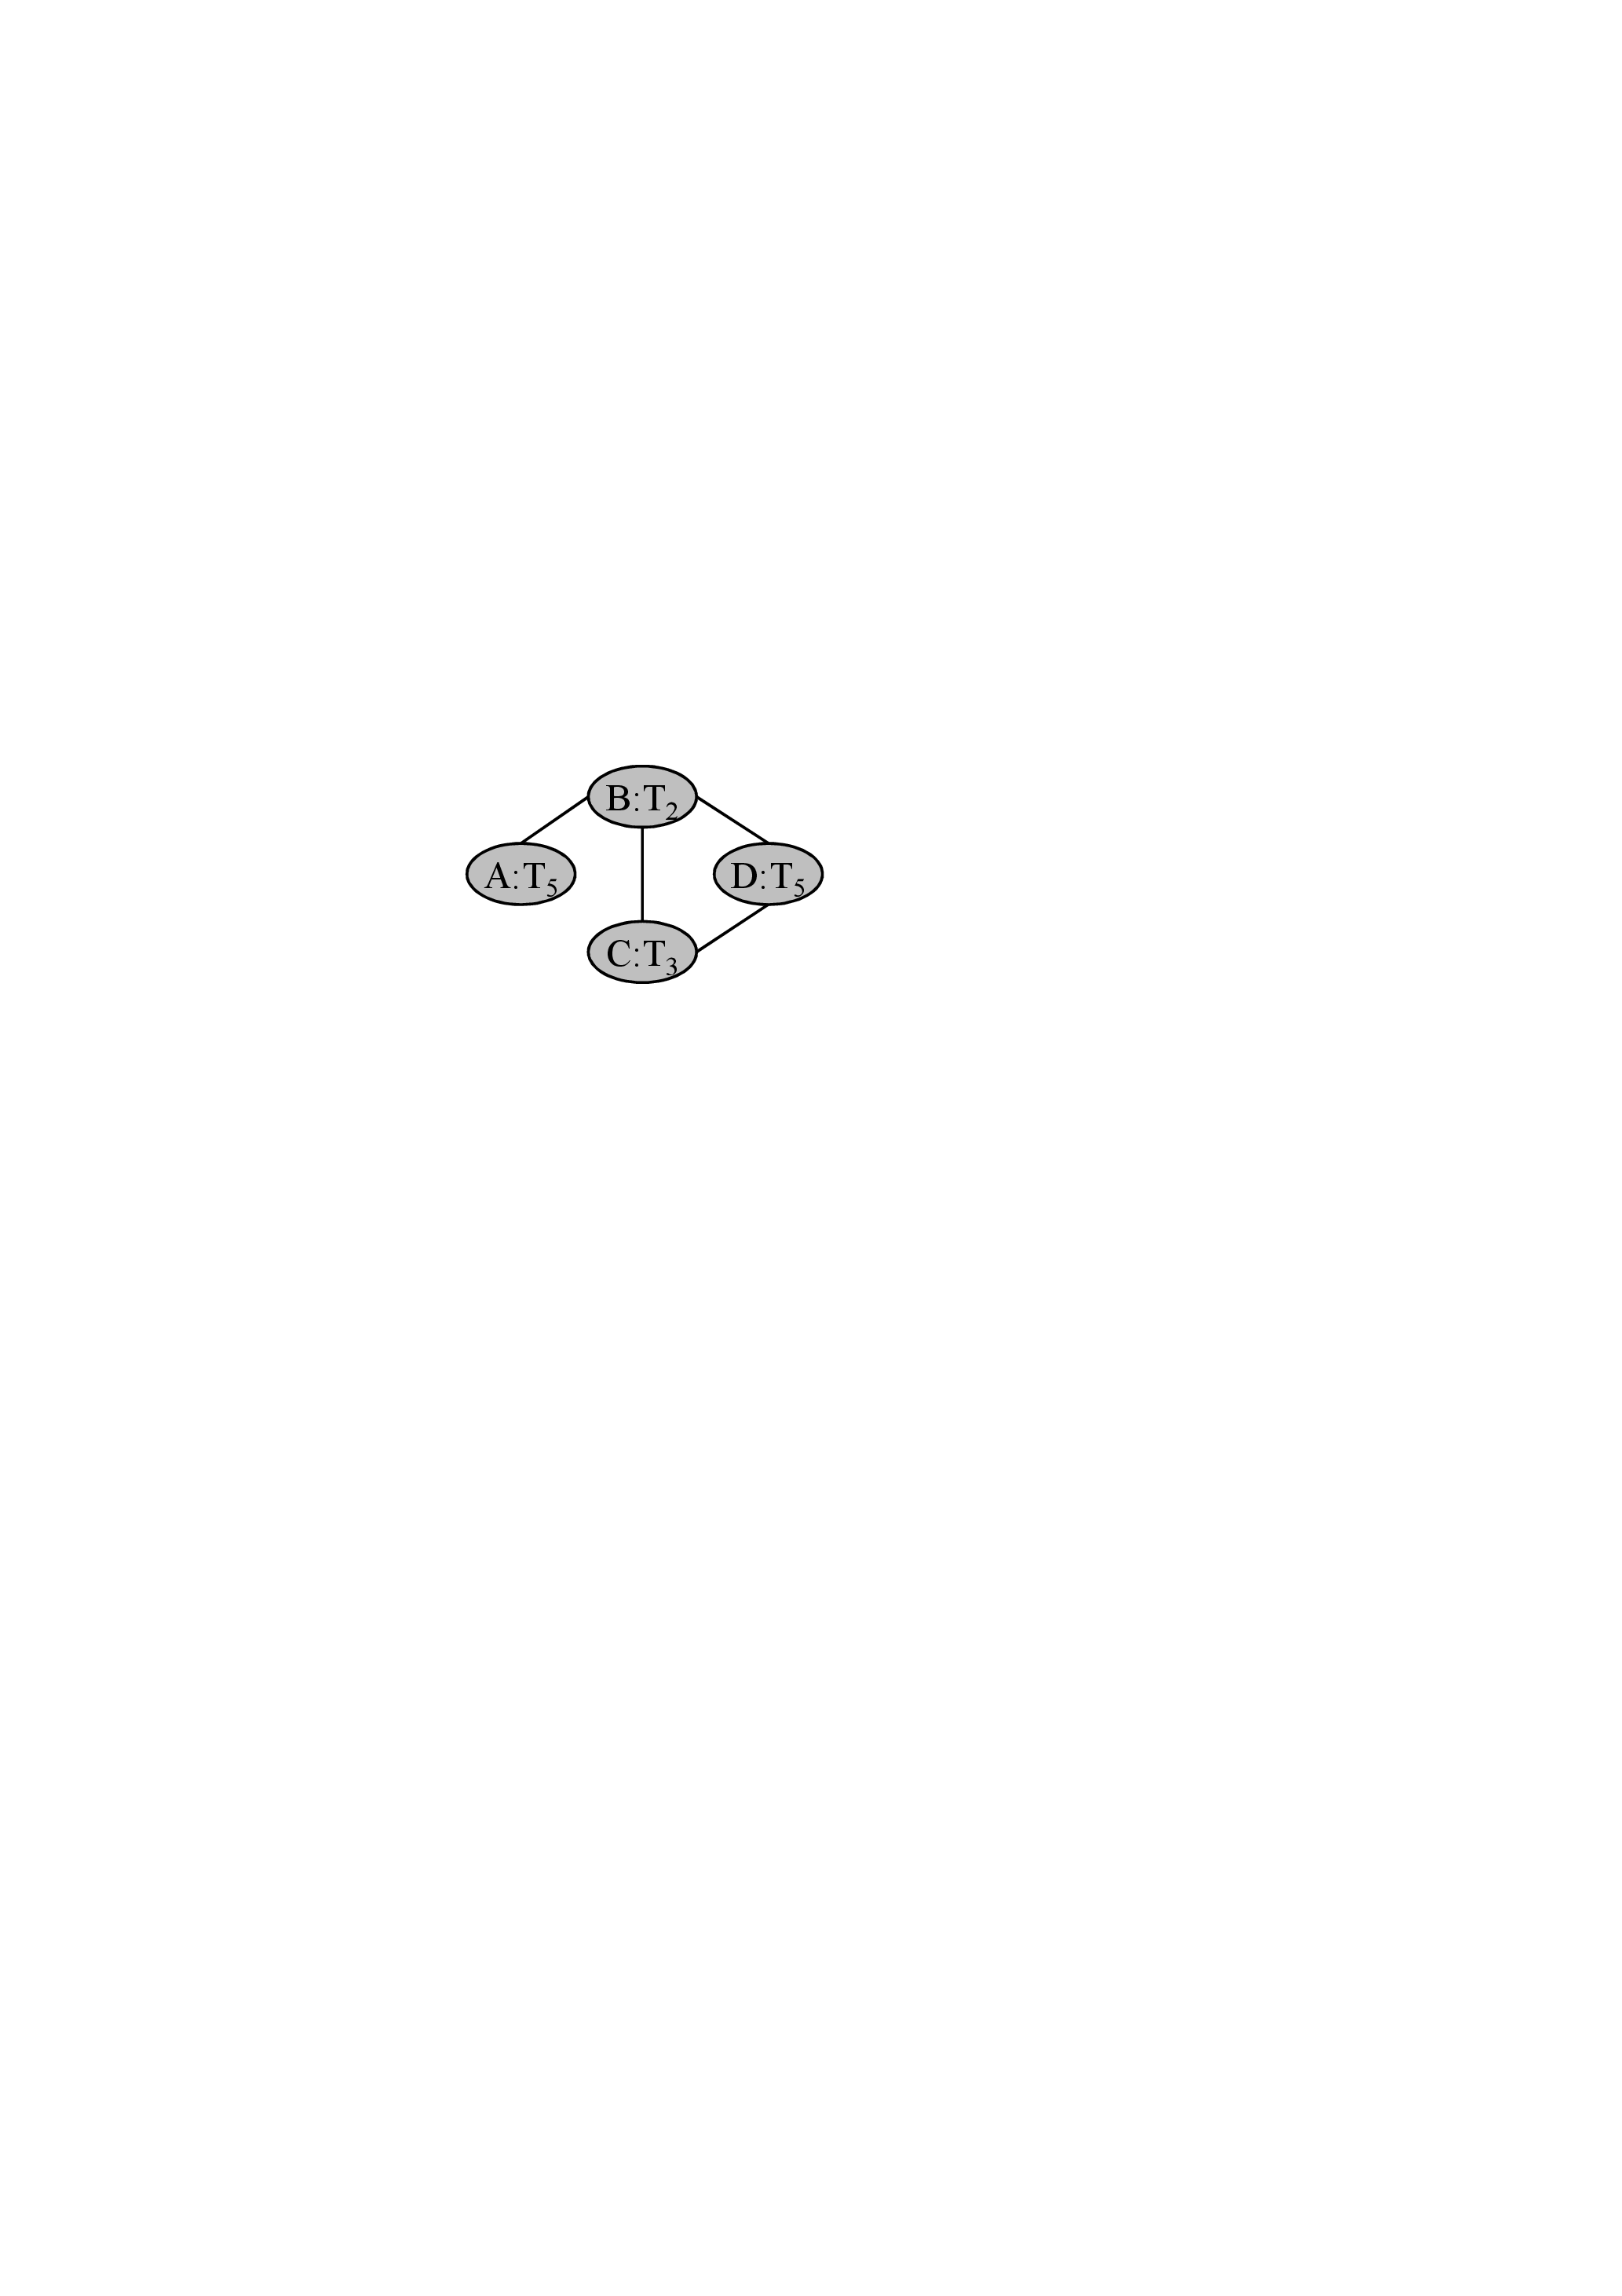}}
    \hspace{0.04\textwidth}
	\subfloat[]{\includegraphics[width=0.16\textwidth]{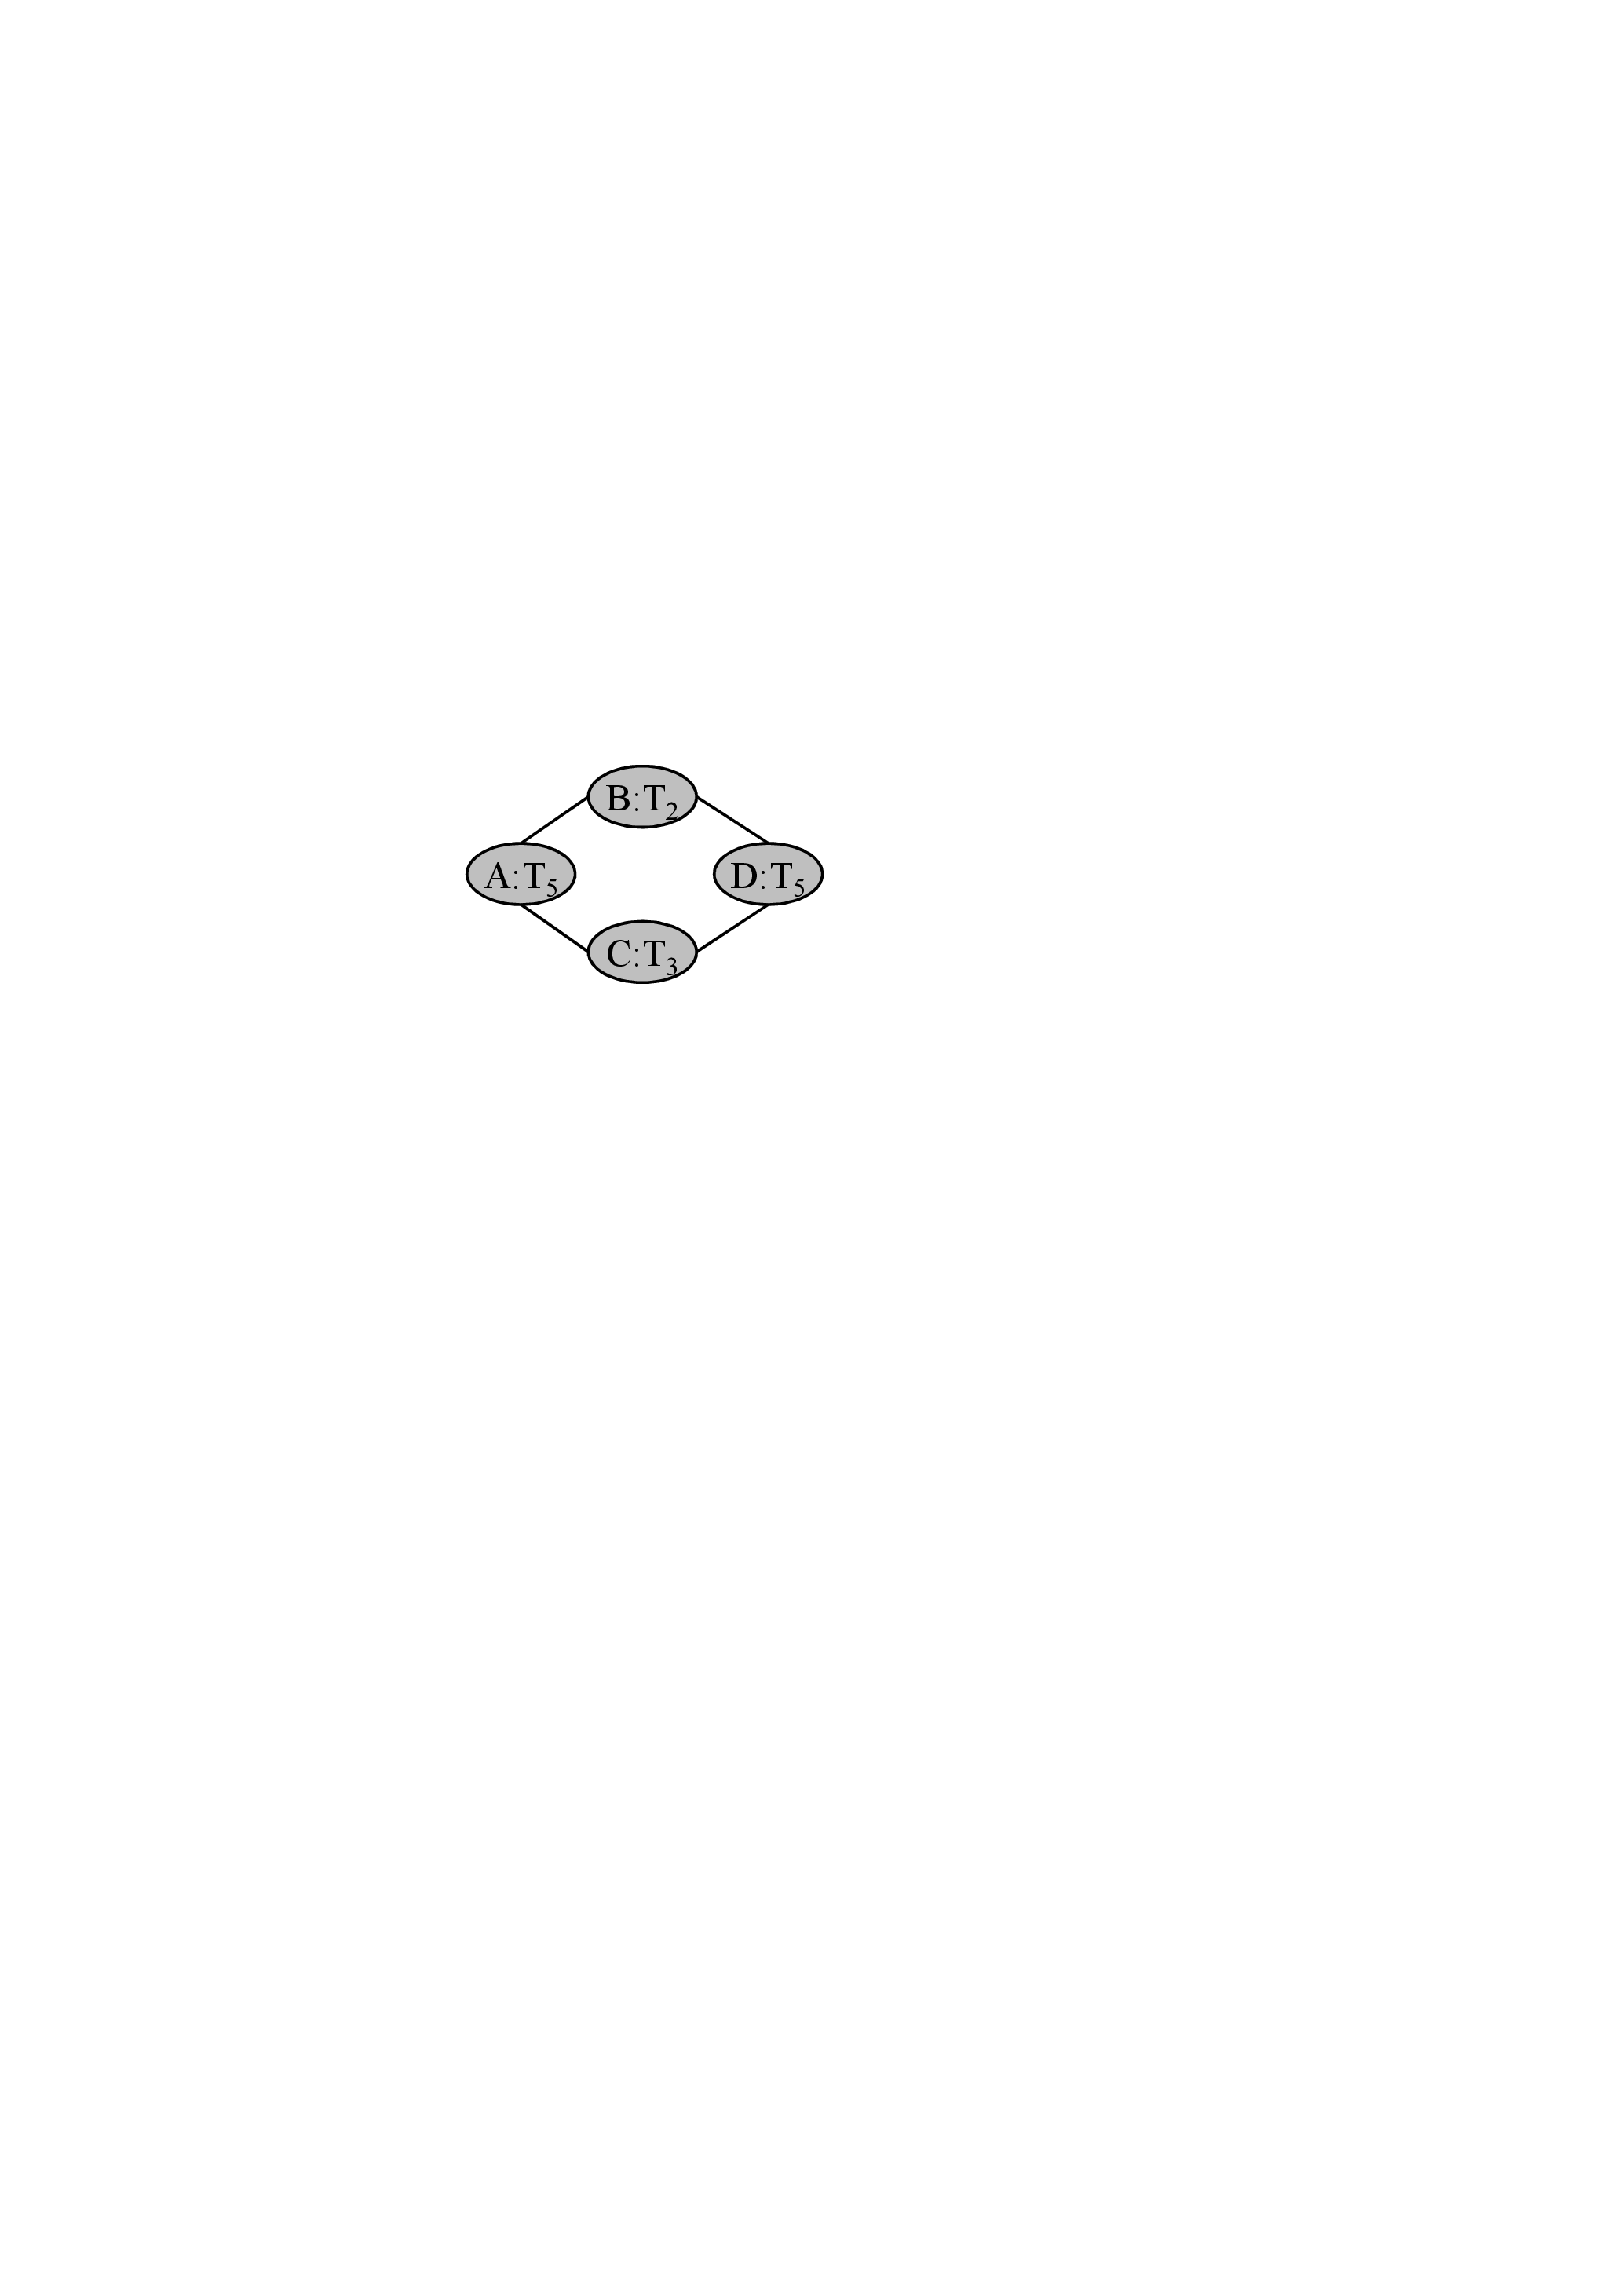}}
	\caption{Merging edge removal: (a) disconnecting $A$ and $C$ removes the merging edge between $A$ and $D$ in Fig. \ref{fig:s_ME}(b); (b) disconnecting $B$ and $C$ removes the merging edge between $A$ and $D$ in Fig. \ref{fig:s_ME}(b).}
	\label{fig:s_MEV}
\end{figure}

\subsubsection{Token Splitting}

\begin{algorithm}[bt!]
\caption{Token Splitting}
\label{alg:s_TSPLIT}
\begin{algorithmic}[1]
  \REQUIRE One TECG $\mathcal{G^{TC}}$ with TG $\mathcal{G^T}$ and CG $\mathcal{G^C}$, token $T_{victim}$ to be split
  \FORALL{$T_{ad} \in V^\mathcal{T}_{ad}(T_{victim})$}
    \STATE $V^\mathcal{T}_{ad}(T_{ad}) := V^\mathcal{T}_{ad}(T_{ad}) - \{T_{victim}\}$;
  \ENDFOR
  \STATE Apply BFS to find the connected component set $S^{CONNECT} \in V^\mathcal{C}_t(T_{victim})$ connected by merging edges of $T_{vicrim}$;
  \FORALL{Connected component $cc \in S^{CONNECT}$}
    \STATE Generate and insert one token $T_{extra}$ in $\mathcal{G^T}$;
    \STATE $V^\mathcal{C}_t(T_{extra}) := \emptyset$;
    \STATE $V^\mathcal{T}_{ad}(T_{extra}) := \emptyset$;
    \FORALL{ CG vertex $v^c \in cc$}
      \STATE $token(v^c) := T_{extra}$;
      \STATE $V^\mathcal{C}_t(T_{extra}) := V^\mathcal{C}_t(T_{extra}) \cup \{v^c\}$;
      \FORALL{Adjacent CG vertex $v^c_{ad}$ of $v^c$}
        \STATE $V^\mathcal{T}_{ad}(T_{extra}) := V^\mathcal{T}_{ad}(T_{extra}) \cup \{token(v^c_{ad})\}$;
        \STATE $V^\mathcal{T}_{ad}(token(v^c_{ad})) := V^\mathcal{T}_{ad}(token(v^c_{ad})) \cup \{T_{extra}\}$;
      \ENDFOR
    \ENDFOR
  \ENDFOR
  \STATE Remove $T_{victim}$ from $\mathcal{G^T}$;
\end{algorithmic}
\end{algorithm}

\begin{figure}[bt!]
	\centering
    %\subfloat[]{\includegraphics[width=0.25\textwidth]{fig/s_TSPIT1.eps}}
    %\subfloat[]{\includegraphics[width=0.15\textwidth]{fig/s_TSPIT1T.eps}}
	%\subfloat[]{\includegraphics[width=0.25\textwidth]{fig/s_TSPIT2.eps}}
	%\subfloat[]{\includegraphics[width=0.15\textwidth]{fig/s_TSPIT2T.eps}}
	%\subfloat[]{\includegraphics[width=0.25\textwidth]{fig/s_TSPIT3.eps}}
	%\subfloat[]{\includegraphics[width=0.15\textwidth]{fig/s_TSPIT3T.eps}}	
    \subfloat[]{\includegraphics[width=0.37\textwidth]{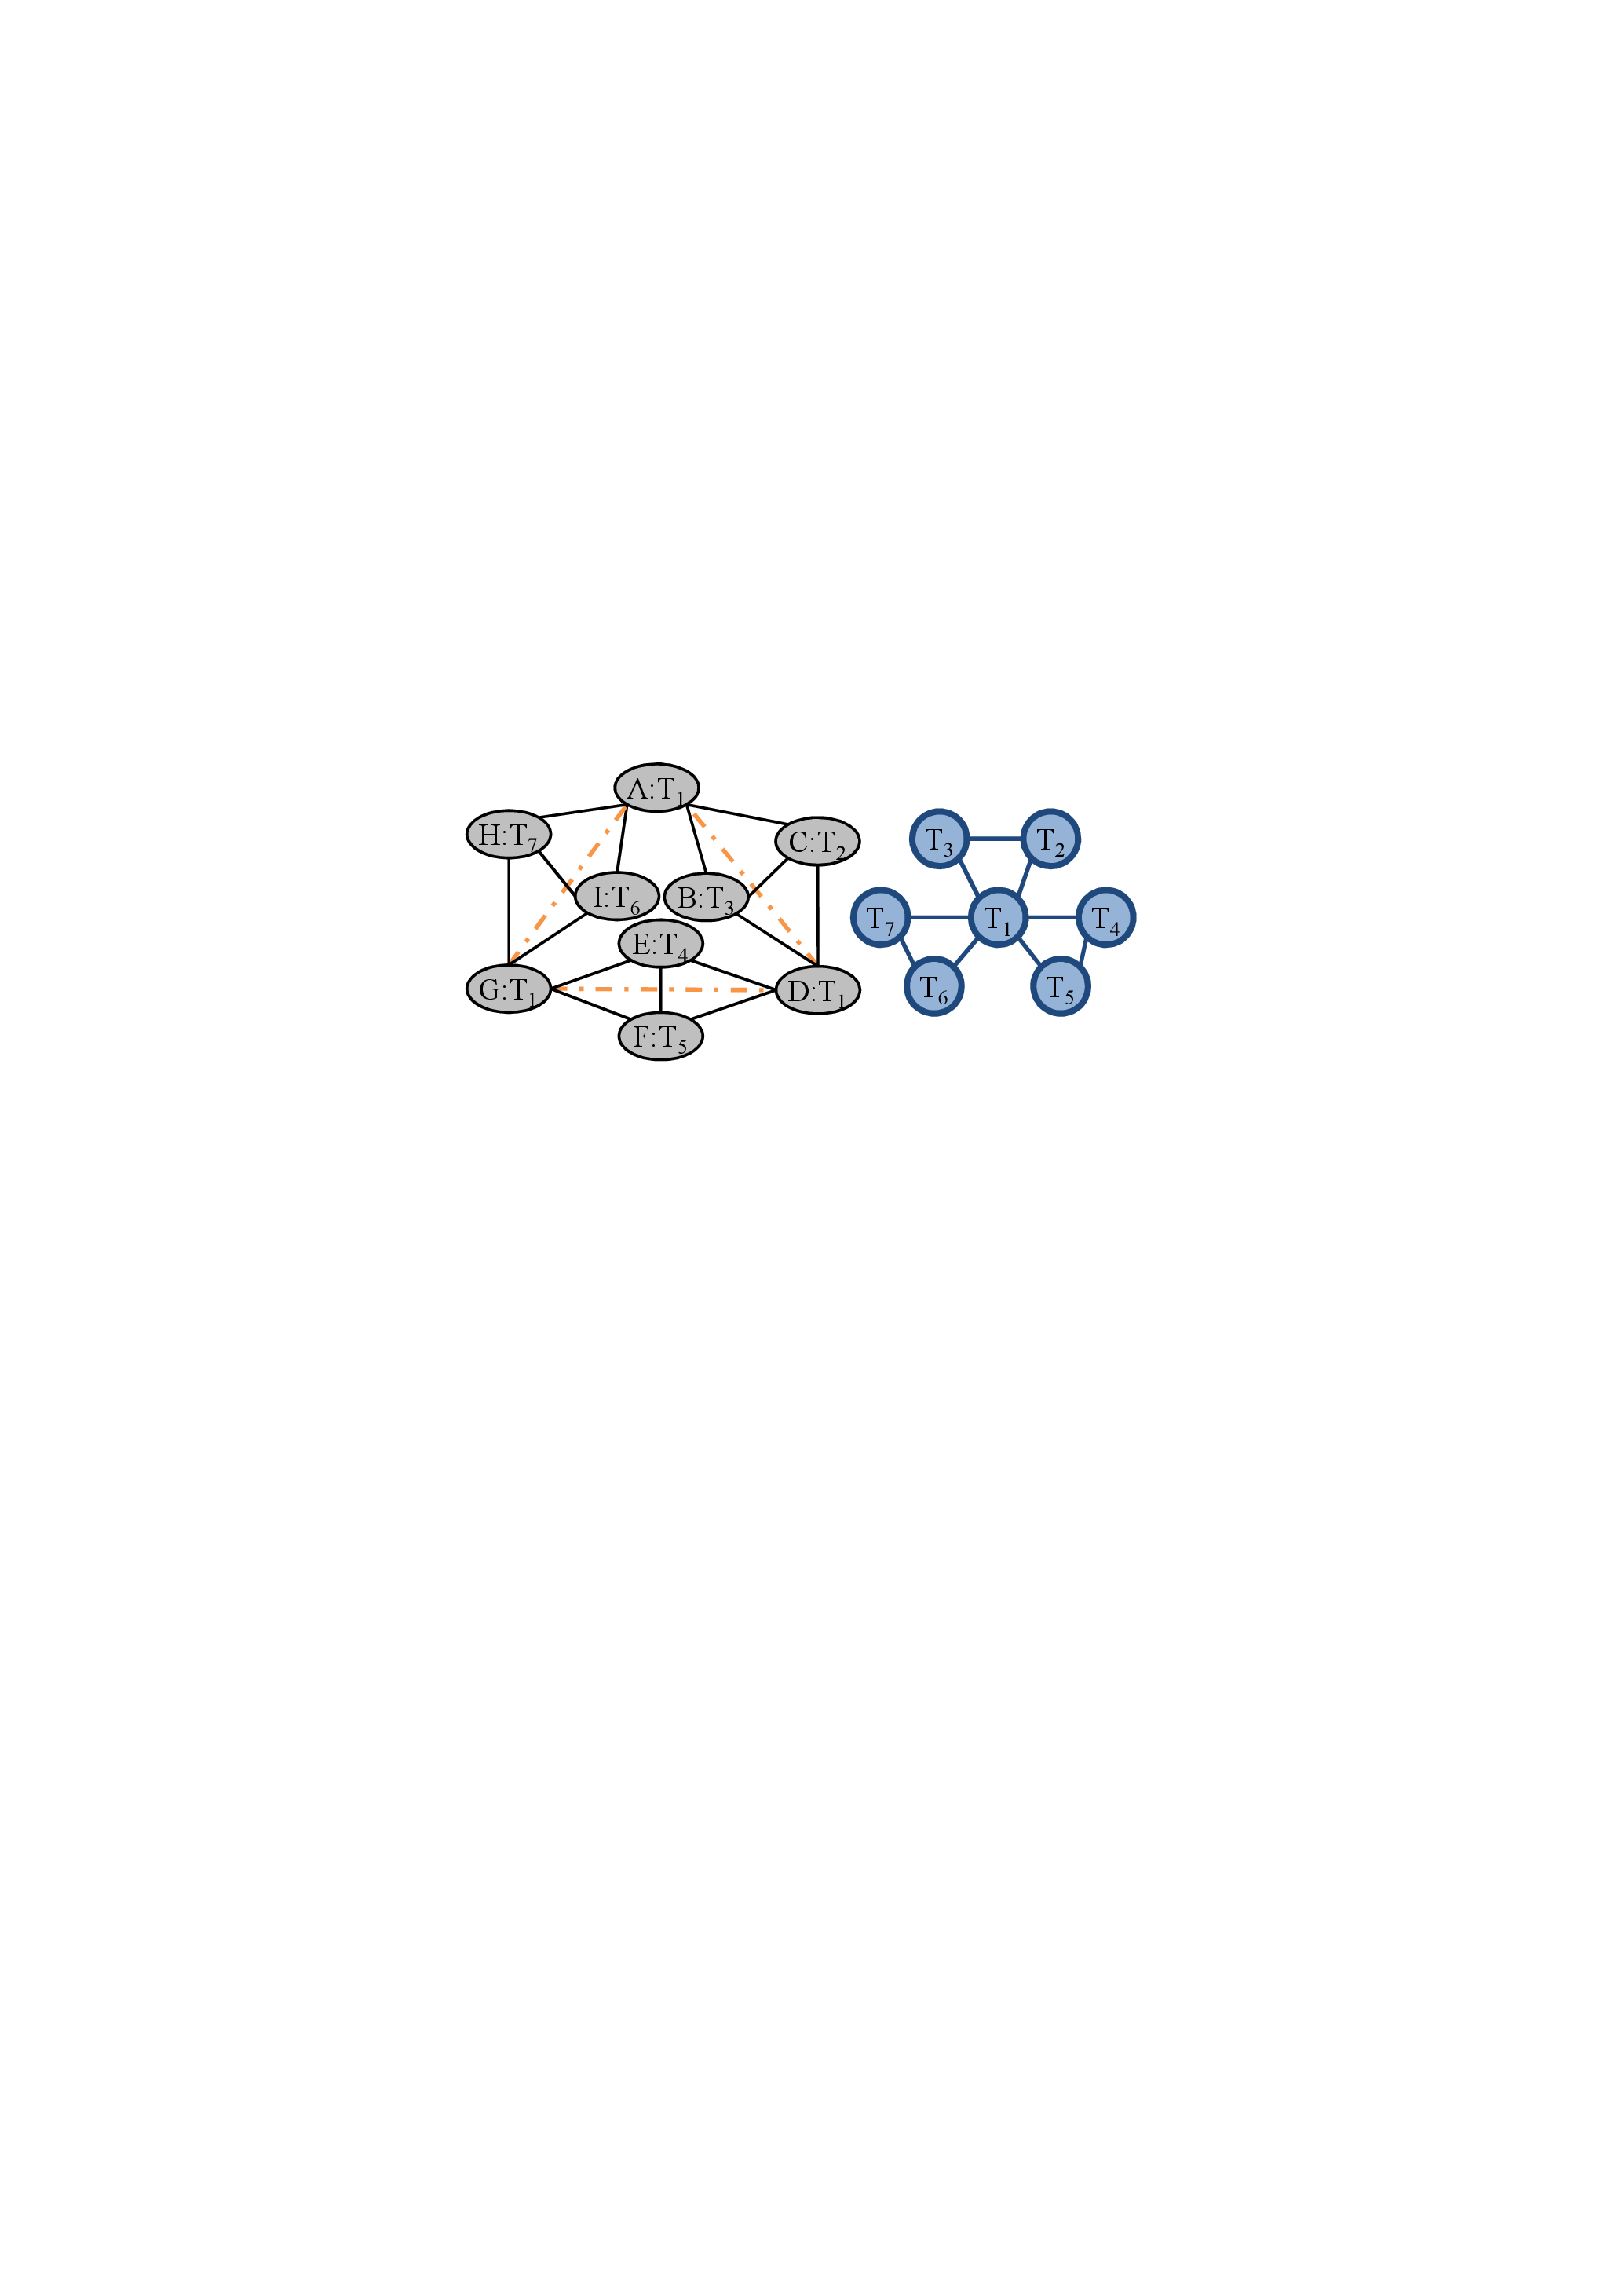}}
	
    \subfloat[]{\includegraphics[width=0.37\textwidth]{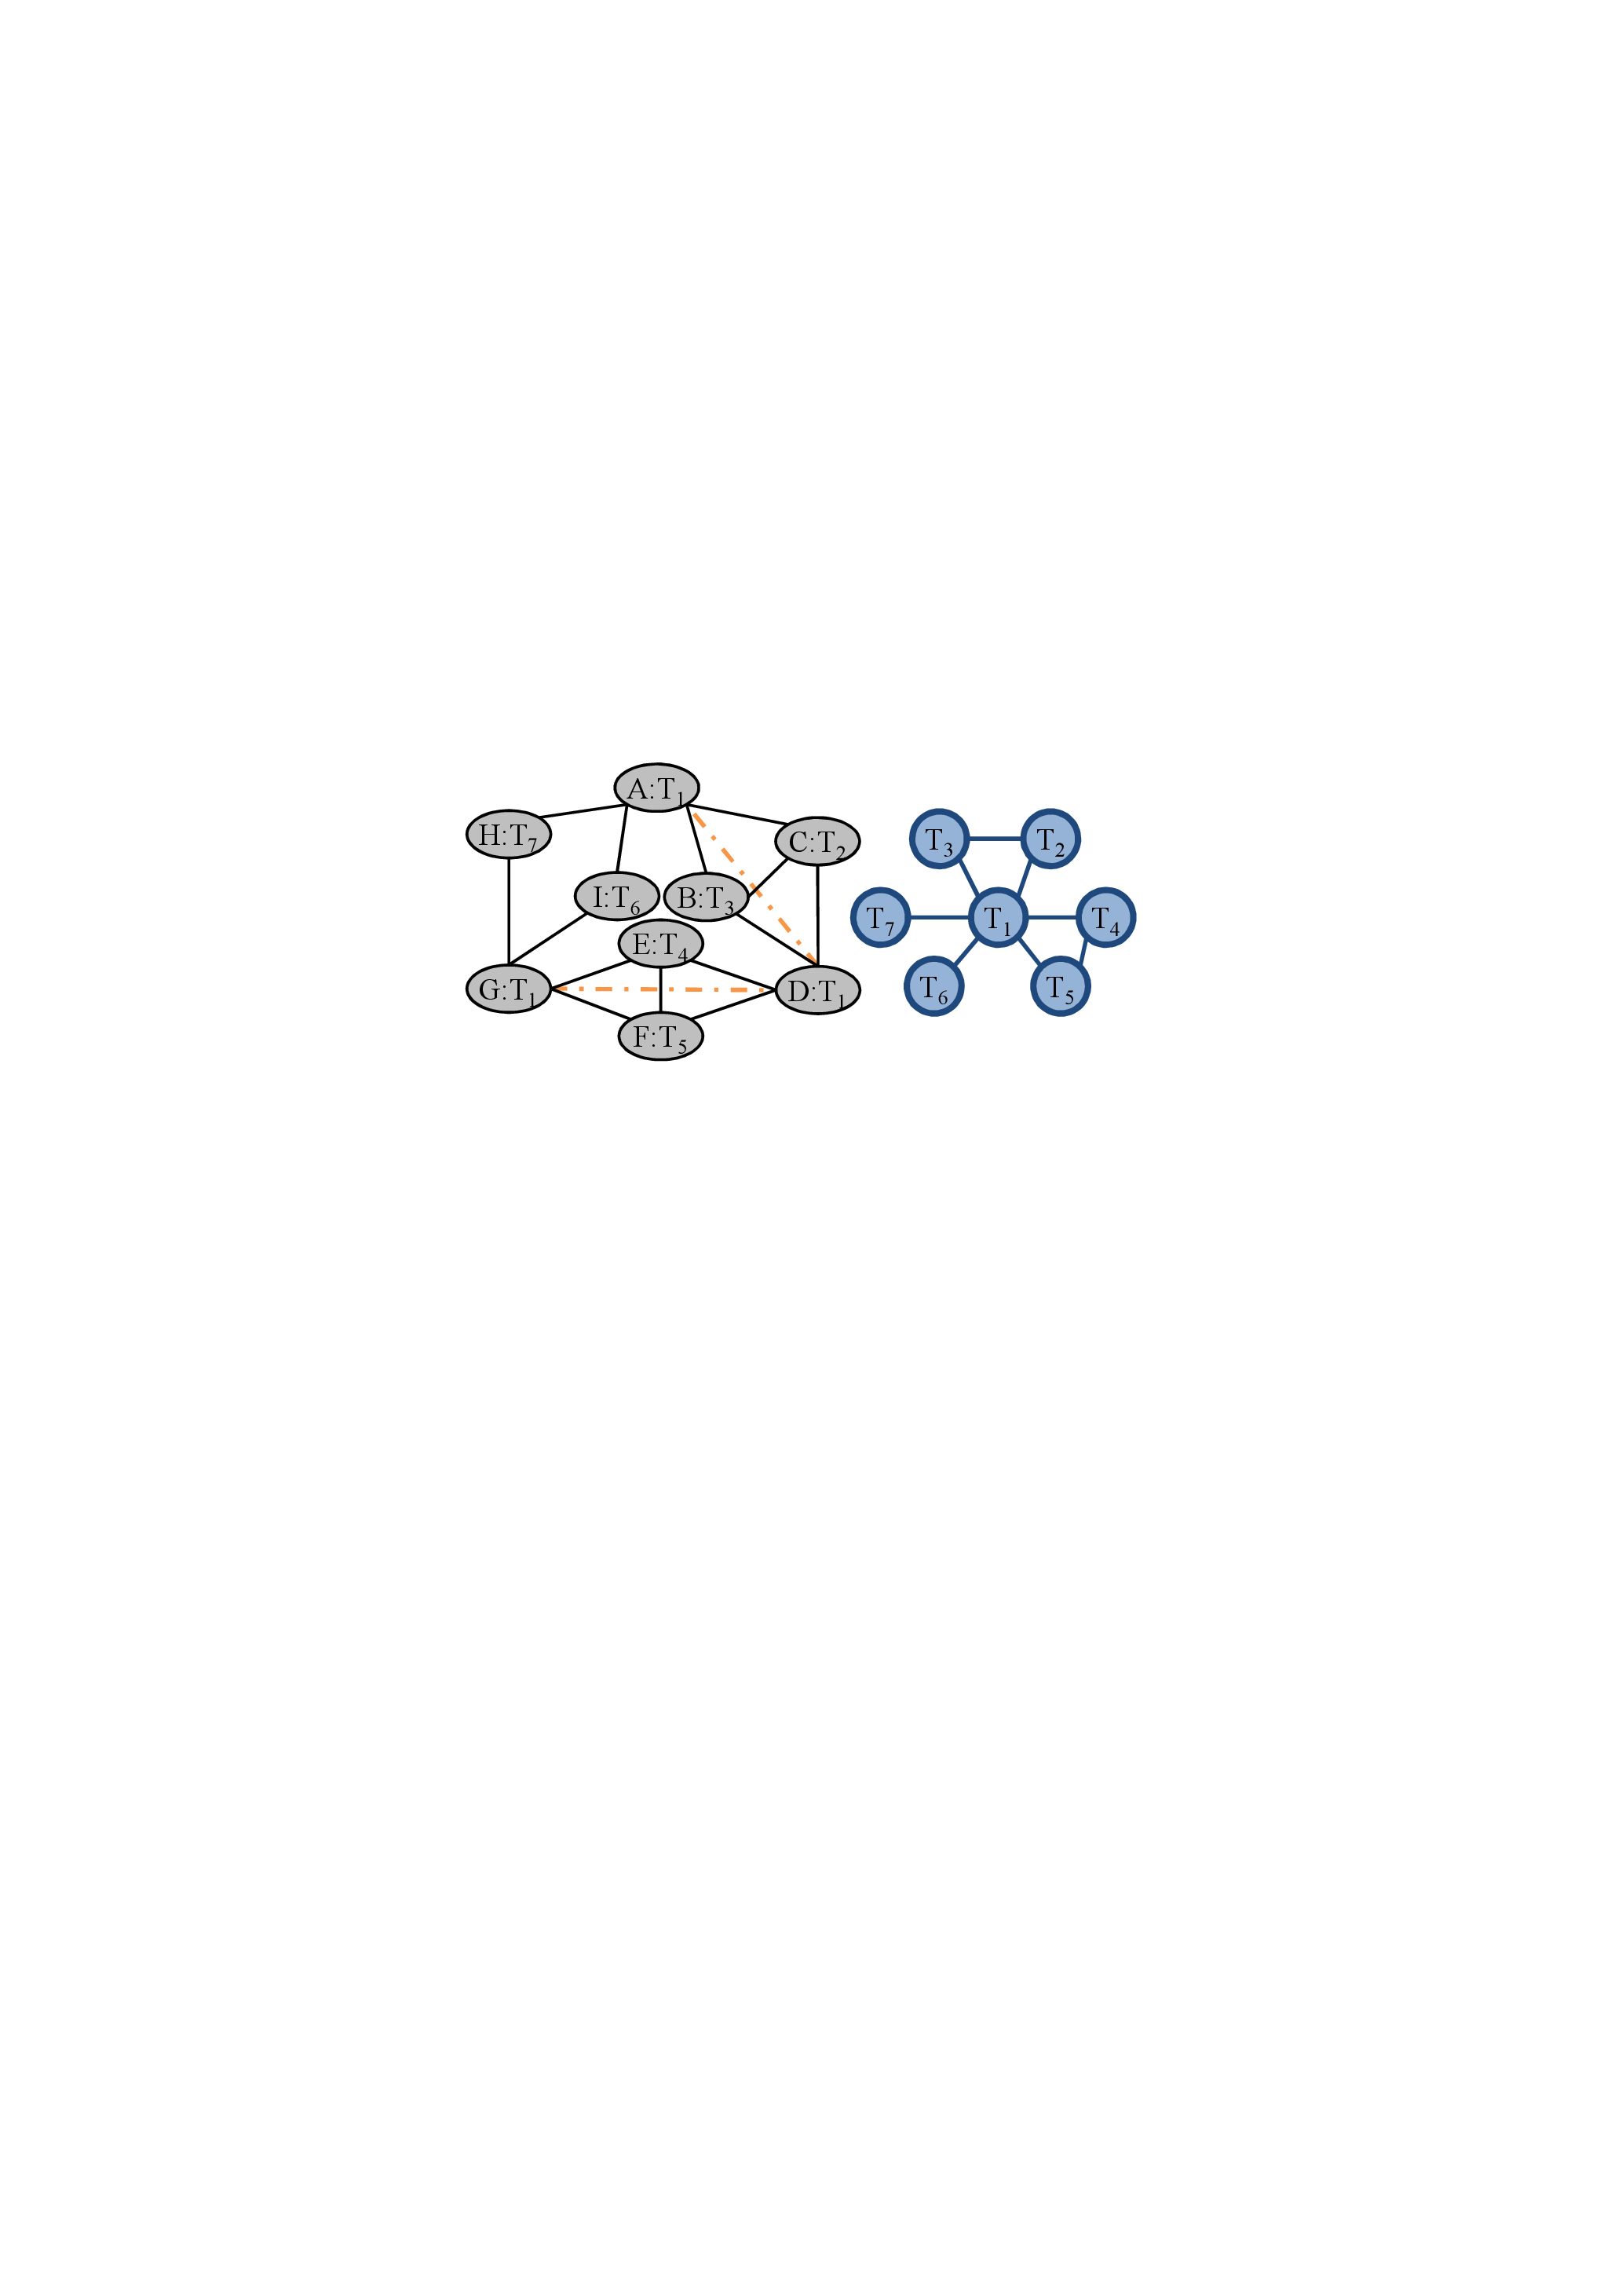}}
	
    \subfloat[]{\includegraphics[width=0.38\textwidth]{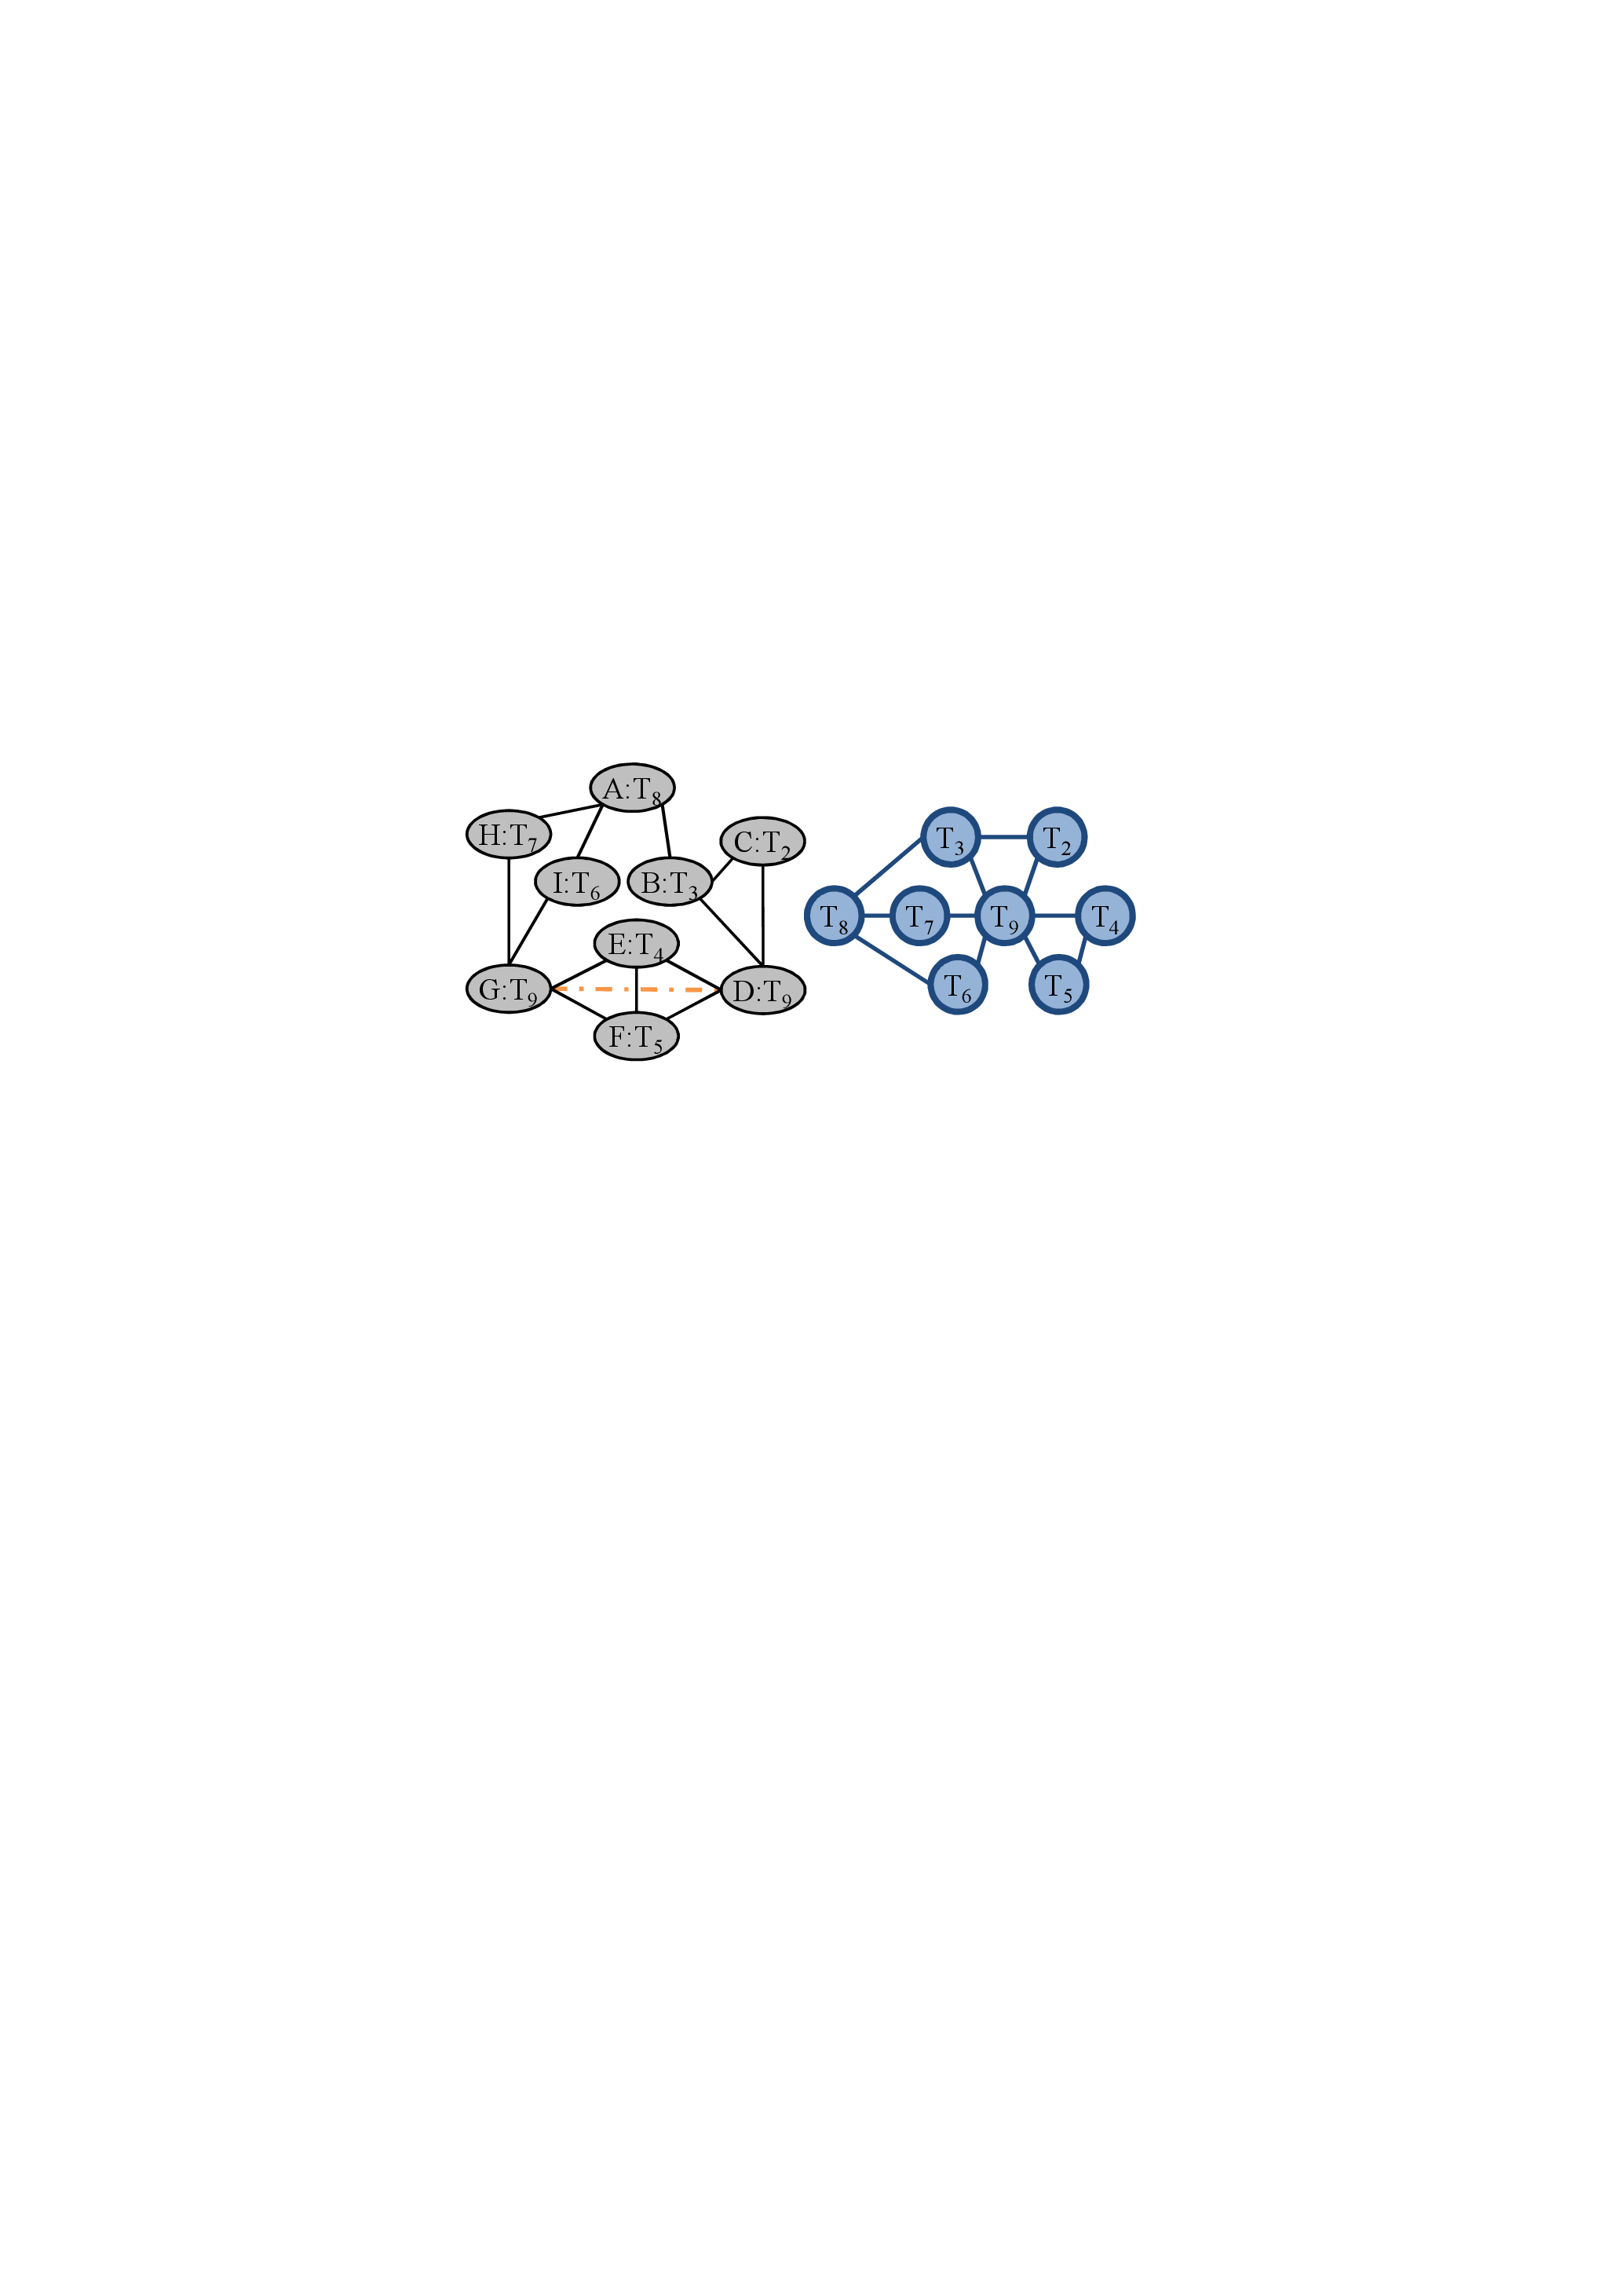}}
	\caption{Token splitting: (a) one TECG where $A$, $D$, and $G$ are connected by merging edges due to $T_1$; (b) disconnecting $I$ and $H$ removes the merging edge between $A$ and $G$; (c) disconnecting $A$ and $C$ removes the merging edge between $A$ and $D$, resulting in $token(A)$ must differ from $token(G)$ and $token(D)$.}
	\label{fig:s_TSPLIT}
\end{figure}

For each token $T_i \in V^\mathcal{T}$, any two vertices, such as $v^c_i \in V^\mathcal{C}_t(T_i)$ and $v^c_j \in V^\mathcal{C}_t(T_i)$, connect to each other by merging edges of $T_i$.
When $v^c_i$ and $v^c_j$ cannot connect to each other by merging edges of $T_i$ after removing edges in CG, $T_i$ needs to be split into at least two tokens.
The connectivity of merging edges can be checked by applying depth-first search (BFS).
Algorithm \ref{alg:s_TSPLIT} shows the algorithm of token splitting.
Firstly, the adjacent token $T_{ad} \in V^\mathcal{T}_{ad}(T_{victim})$ and $T_{victim}$ is disconnected (lines 1--3).
BFS is then applied to find the connected component set $S^{CONNECT}$ where all vertices in each component $cc \in S^{CONNECT}$ are connected by merging edges of $T_i$ (line 4).
%Then, $T_{victim}$ is split into $|S^{CONNECT}|$ tokens.
For each connected component $cc \in S^{CONNECT}$, one extra token $T_{extra}$ is generated and inserted in TG.
For each CG vertex $v^c \in cc$, $token(v^c)$ is assigned to $T_{extra}$ (lines 5--11).
The adjacent tokens of $T_{extra}$ is updated based on the tokens of all adjacent vertices of $v^c$ (lines 12--15).
Finally, $T_{victim}$ is removed from TG (line 18).

Figure \ref{fig:s_TSPLIT}(a) depicts one TECG containing one CG with nine vertices, fifteen edges, and three merging edges of $T_1$ and one TG with seven tokens and nine edges.
$A$, $D$, and $G$ connect to each other by the three merging edges of $T_1$ because they are assigned to $T_1$.
After disconnecting $H$ and $I$, the merging edge of $T_1$ between $A$ and $G$ is removed, and $T_6$ and $T_7$ are also disconnected as shown in Fig. \ref{fig:s_TSPLIT}(b).
$A$, $D$, and $G$ still connect to each other by the remaining two merging edges of $T_1$.
Then, disconnecting $A$ and $C$ removes the merging edge of $T_1$ between $A$ and $D$, sequentially generating two connected component in terms of the connectivity of merging edges of $T_1$.
Therefore, $T_1$ is split into $T_8$ and $T_9$, resulting in that $A$ is reassigned to $T_8$ while $D$ and $G$ are reassigned to $T_9$.
The adjacent tokens of $T_8$ and $T_9$ are updated according to the connection in CG.
Figure \ref{fig:s_TSPLIT}(c) displays the TECG after splitting $T_1$ into $T_8$ and $T_9$.
